# Supplementary material for: Tackling Combinatorial Distribution Shift: A Matrix Completion Perspective
Source: arXiv:2307.06457 source file (2023-07-28)
Supplement: Supplementary file 1 [file assumptions_app.tex]

%!TEX root = ../colt_main.tex

\section{Justification of Assumptions}

\subsection{Class of Functions}
\begin{prop} Let $\hst(x,y) = \sum_{i,j=1}^{\infty} a_{i,j}\phi_i(x)\psi_j(x)$, and suppose that the following terms are finite:
\begin{align*}
M_x:= \sup_{i \ge 1}\sup_{x \in \xspac}|\phi_i(x)| , \quad M_y := \sup_{j \ge 1}\sup_{y \in \yspace}|\psi_j(y)| , \quad C:= \sum_{i,j \ge 1} |a_{ij}|.
\end{align*}
Then, there exists embeddings $\fst:\xspac \to \ell_2(\N)$ and $\gst:\yspace \to \ell_2(\N)$ such that $\hst(x) = \langle \fst,\gst \rangle$ and  
\begin{align*}
\sup_{x \in \xspac} \|\fst(x)\|_{\ell_2} \le M_x\sqrt{C}, \quad \sup_{y \in \yspace} \|\gst(y)\|_{\ell_2} \le M_y\sqrt{C}
\end{align*}
\end{prop}
\begin{proof}
Let  $\iota: \N \times \N \to \N$ be a bijective mapping such that $\iota(j,i) \le \max\{i,j\}^2$ (such an indexing mapping is easy to construct by induction on $\max\{i,j\}$). Define $(i_k,j_k)$ so that $\iota(i_k,j_k) = k$ (since $\iota$ is a bijection, these indices are unique).
\begin{align*}
\fst_{k}(x) = \sqrt{a_{i_kj_k}}\phi_{i_k}(x), \quad \gst_{k} = \sqrt{a_{i_kj_k}}\psi_{i_k}(x)
\end{align*}
Then, 
\begin{align*}
\sum_{k\ge 1}\fst_{k}(x)\gst_{k} = \sum_{k}a_{i_kj_k}\phi_{i_k}(x)\psi_{j_k}(x) =  \sum_{i,j}a_{i,j}\phi_{i}(x)\psi_{j}(y) = \hst(x,y), 
\end{align*}
where the second equality holds since $\iota$ is a bijection. Moreover, we have
\begin{align*}
\|\fst(x)\|_{\ell_2}^2 = \sum_{k\ge 1}|\fst_{k}(x)|^2 = \sum_{k\ge 1}|a_{i_kj_k}|\phi_{i_k}(x)^2 \le M_x^2\sum_{k\ge 1}|a_{i_kj_k}| = M_x^2\sum_{i,j \ge 1}|a_{i,j}| = C M_x^2,
\end{align*}
where again we used that $\iota$ is a bijection. 
\end{proof}

\subsection{On the Balancing Assumption \label{app:balancing_asm}}
