# Supplementary material for: Tackling Combinatorial Distribution Shift: A Matrix Completion Perspective
Source: arXiv:2307.06457 source file (2023-07-28)
Supplement: Supplementary file 2 [file lin_alg_old.tex]

%!TEX root = ../main.tex

\section{Linear Algebra}
\subsection{Proof of \Cref{prop:projected_factor}}
 Define $\btilA := \bstPk \bhatA$ and $\btilB := \bstQk \bhatB$, where again $\bstPk$ (resp. $\bstQk$). are the projections on the left (resp. right) top-$r$ singular subspaces of $\bstM$. We restate the proposition as follows
\propprojectedfactor*
Throughout, we use
\begin{align}
\|\btilM - \bstMk\|_{\mathrm{nrm}} = \|\bstPk(\bhatM - \bstM)\bstQk\|_{\mathrm{nrm}} \le \|\bhatM - \bstM\|_{\mathrm{nrm}}, \quad \mathrm{nrm} \in \{\mathrm{op},\mathrm{fro}\}. \label{eq:norm_equivalence}
\end{align}
\newcommand{\bd}{\mathbf{d}}

Write out $\btilA = \bU_A \bSigma_A \bV_A^\top$ and $\btilB = \bU_B \bSigma_B \bV_B^\top$ as a compact SVD, (b)  $\bQ = \bV_B^\top \bV_A$. Define
\begin{align*}
\bcircA := \bU_A \bSigma_A  \in \R^{n \times r}, \quad \bcircB := \bU_B  \bSigma_B \bQ \in \R^{m \times r}
\end{align*}
Lastly, introduce indicator vectors $\bd_{A}, \bd_{B} \in \{0,1\}^2$ which pick out the $\max\{\sigma_i(\bA),\sigma_i(\bB)\}$ in the sense that 
\begin{align*}
\bd_{A}[i], \bd_{B}[i] \in \{0,1\}, \quad \bd_{A}[i] +  \bd_{B}[i] = 1, \quad \sigma_i(\bcircA)\bd_{A}[i] + \sigma_i(\bcircB)\bd_{B}[i] = \max\{\sigma_i(\bcircA),\sigma_i(\bcircB)\}.
\end{align*}
We let $\bD_{A},\bD_{B}$ be the binary, diagonal matrices with $\bd_{A},\bd_B$ on the diagonal. 

\begin{lemma}\label{lem:exists_fact} Suppose that for some $\gamma \in (0,1)$, $\epsop \le (1-\gamma)\sigma_r(\bstM)$. Then there exists matrices $\bstilAr,\bstilBr$ such that $\bstilAr(\bstilBr)^\top = \bstMk$, and 
\begin{align*}
2\|\btilA  - \bstilAr\|_{\fro}^2 +  \|\btilB - \bstilBr\|_{\fro}^2 \le 2\epsfro^2 \cdot \frac{(2-\gamma)\cproc\|\bstM\|_{\op}}{\gamma^2 \sigma_r(\bstM)^2} + 2\trace(\bSigma_B (\eye_{r_0} - \bQ \bQ^\top ) \bSigma_B),
\end{align*}
\end{lemma}

\begin{lemma}\label{lem:remainder_term}
 \begin{align*}
 \trace(\bSigma_B (\eye_{r_0} - \bQ \bQ^\top ) \bSigma_B) \le \frac{8\epsfro \fronorm{\bhatM}}{(1-\gamma)\sigma_r(\bstM)}
 \end{align*}
 \end{lemma}
 In conclusion, taking $\gamma \le 1$, wehave
 \begin{align*}
 2\|\btilA  - \bstilAr\|_{\fro}^2 +  \|\btilB - \bstilBr\|_{\fro}^2 \le \frac{4\epsfro \|\bhatM\|_{\fro}}{(1-\gamma) \sigma_r(\bstM)}\left(4 + \epsfro\cdot\frac{\cproc\|\bstM\|_{\op}}{\|\bhatM\|_{\fro}(1-\gamma)\sigma_r(\bstM)}\right)
 \end{align*}

\subsubsection{Proof of \Cref{lem:exists_fact}}
    \begin{proof} 
    \begin{claim}\label{claim_Eclaim} We have
    \begin{align*}
    \btilA = \bcircA \bV_A^\top, \quad  \btilB =  \bcircB \bV_A^\top + \bE,
    \end{align*} 
    where
    $\|\bE\|_{\fro}^2 = \trace(\bSigma_B (\eye_{r_0} - \bQ \bQ^\top  ) \bSigma_B)$. 
    \end{claim}
    \begin{proof}
    We have
    \begin{align*}
    \btilA &= \bcircA \bV_A^\top\\
    &= \bU^\top \bSigma_A (\bD_A + \bD_B)\bV_A^\top\\
    &= \bU^\top \bSigma_A \bD_A \bV_A^\top + \bU^\top \bSigma_A \bD_B \bV_A^\top\\
    &= \bU^\top \bSigma_A (\bD_A \bV_A^\top + \bD_B \bV_B^\top) + \bU^\top \bSigma_A \bD_B \bV_A^\top
    \end{align*}
    \begin{align*}
    \btilA &= \bcircA \bV_A^\top \\
    \btilB &=  \bcircB \bV_A^\top + \bU_B \bSigma_B (\bQ\bV_A^\top - \bV_B^\top) \\
    &=  \bcircB \bV_A^\top + \bU_B \bSigma_B (\bV_B^\top\bV_A\bV_A^\top - \bV_B^\top) \\
    &=  \bcircB \bV_A^\top + \bU_B \bSigma_B \bV_B^\top(\bV_A\bV_A^\top - \eye_{r_0}) 
    \end{align*}
    Lastly, we compute
    \begin{align*}
    \|\bU_B \bSigma_B \bV_B^\top(\eye_{r_0} - \bV_A\bV_A^\top - )\|_{\fro}^2 &= \|\bSigma_B \bV_B^\top( \eye_{r_0} - \bV_A\bV_A^\top - )\|_{\fro}^2\\
    &=  \trace(\bSigma_B \bV_B^\top(\eye_{r_0} - \bV_A\bV_A^\top - )(\eye_{r_0} - \bV_A\bV_A^\top )^\top \bV_B \bSigma_B)\\
    &\overset{(i)}{=}  \trace(\bSigma_B \bV_B^\top(\eye_{r_0} - \bV_A\bV_A^\top ) \bV_B \bSigma_B)\\
    &\overset{(ii)}{=}  \trace(\bSigma_B (\eye_{r_0} - \bV_B^\top\bV_A \cdot \bV_A^\top\bV_B^\top ) \bSigma_B)\\
    &=  \trace(\bSigma_B (\eye_{r_0}  - \bQ \bQ^\top ) \bSigma_B),
    \end{align*}
    where $(i)$ uses that $ \eye_{r_0}- \bV_A\bV_A^\top$ is an orthogonal projection, and thus symmetric and idempotenent and $(ii)$ uses that $\bV_B^\top \bV_B  = \eye_r$ since $\bV_B \in \R^{r \times r_0}$ (with $r_0 \ge r$) has orthonormal columns. The claim follows. 
    \end{proof}

    \begin{claim}\label{claim:balance_claim} Suppose $\epsop \le \gamma \sigma_r(\bstM)$. Then,given a balanced factorization $\btilM = \bsqA\bsqB^\top$, there exists an $\bR \in \GL r$ with $\|\bR\|_{\op}^2 \vee \|\bR^{-1}\|_{\op}^2 \le \frac{(2-\gamma)\|\bstM\|_{\op}}{\gamma\sigma_{r}(\bstM)}$ such that 
    \begin{align*}
    \bsqA\bR = \bcircA, \quad \bsqB\bR^{-\top} = \bcircB
    \end{align*}
    \end{claim}
    \begin{proof}
    We have that
    \begin{align*}
     \max\{\|\bcircA\|_{\op},\|\bcircB\|_{\op}\} &= \max\{\|\bSigma_A\|_{\op}, \|\bSigma_B\|_{\op}\|\bQ\|_{\op}\}\\
     &\le \max\{\|\bSigma_A\|_{\op}, \|\bSigma_B\|_{\op}\} = \max\{\|\btilA\|_{\op},\|\btilB\|_{\op}\}\\
     &\le  \max\{\|\bhatA\|_{\op},\|\bhatB\|_{\op}\} = \|\bhatM\|_{\op}^{\half},
     \end{align*}
     where above we used that $ \|\bQ\|_{\op} \le \|\bV\|_{\op}\|\bV_B\|_{\op} \le 1$, and that $\bhatA\bhatB^\top$
     is a balanced factorization of $\bhatM$.  Similarly, letting $\bsqA \bsqB^\top = \btilM$ be a balanced factorization of $\btilM$, we have
     \begin{align*}
     \min\{\sigma_{\min}(\bsqA),\sigma_{\min}(\bsqB)\} = \sigma_{\min}(\btilM)^{\half}
     \end{align*}

     Observe observe that since $\|\btilM - \bstMk\|_{\op} \le \epsop$, for $\epsop \le (1-\gamma\sigma_r(\bstM) = (1-\gamma)\sigma_{r}(\bstMk)$, we have $\sigma_r(\btilM) \ge \gamma\sigma_{r}(\bstMk)$. In particular, $\rank(\btilM) = r$, and thus there exists an $\bR \in \GL(r)$ for which $\bsqA \bR = \bcircA$ and $\bsqB \bR^{-\top} = \bcircB$. Thus, 
     \begin{align*}
     \|\bR\|_{\op}  = \|\bsqA^{\dagger}\bA\|_{\op} \le \frac{\|\bA\|}{\sigma_{\min}(\bsqA)} = (\frac{\|\bhatM\|_{\op}}{\sigma_{\min}(\btilM)})^{\half}.
     \end{align*}
     and similarly, 
     \begin{align*}
     \|\bR^{-1}\|_{\op} = \|\bR^{-\top}\|_{\op}  = \|\bsqB^{\dagger}\bB\|_{\op} \le \frac{\|\bB\|_{\op}}{\sigma_{\min}(\bsqB)} = (\frac{\|\bhatM\|_{\op}}{\sigma_{\min}(\btilM)})^{\half} \le (\frac{3\|\bstM\|_{\op}}{\sigma_{r}(\bstM)})^{\half}.
     \end{align*}

      Our conditions on $\epsop$ imply $\sigma_r(\btilM) \ge (1-\gamma)\sigma_{r}(\bstMk)$ and $\|\bhatM\|_{\op} \le (2-\gamma)\|\bstM\|_{\op}$ so that
      \begin{align*}
     \|\bR\|_{\op} \vee \|\bR^{-1}\|_{\op}  \le (\frac{(2-\gamma)\|\bstM\|_{\op}}{\gamma\sigma_{r}(\bstM)})^{\half}.
     \end{align*}
     \end{proof}

     Next, we argue that there exists a good balanced factorization of $\btilM$:
     \begin{claim} There exists an orthonormal matrix $\bO \in \bbO(r)$ such that, for $\bR$ in \Cref{claim:balance_claim}, we have
     \begin{align*}
    \|\bcircA  - \bstAk \bO\bR^{-1}\|_{\fro}^2 +  \|\bcircB  - \bstBk \bO \bR^{\top}\|_{\fro}^2 \le  \epsfro^2 \cdot \frac{(2-\gamma)\cproc\|\bstM\|_{\op}}{\gamma^2 \sigma_r(\bstM)^2}, 
    \end{align*}
    provided $\epsop \le \gamma\sigma_r(\bstM)$. 
     \end{claim}
     \begin{proof} 
     Recall $\bstAk,\bstBk$ gives a balanced factorization of $\bstMk$. Hence, for $\epsop \le \gamma\sigma_r(\bstMk) = \gamma \sigma_r(\bstM)$, we have that $\|\btilM - \bstMk\|_{\op} \le (1-\gamma)\sigma_r(\bstM)$, and thus \Cref{lem:proc} ensures that for any balanced factorization $\bsqA \bsqB^\top = \btilM$, there is an $\bO \in \bbO(r)$ for which
    \begin{align*}
    \|\bsqA - \bstAk \bO\|_{\fro}^2 + \|\bsqB - \bstBk \bO\|_{\fro}^2 \le \cproc \frac{\epsfro^2}{\gamma \sigma_r(\bstMk)} =  \cproc \frac{\epsfro^2}{\gamma \sigma_r(\bstMk)}
    \end{align*}
    Hence, letting $\bR$ be as in \Cref{claim:balance_claim}

    \begin{align*}
    \cproc \frac{\epsfro^2}{\gamma \sigma_r(\bstM)} &\ge \|\bcircA \bR - \bstAk \bO\|_{\fro}^2 + \|\bcircB \bR^{-\top} - \bstBk \bO\|_{\fro}^2 \le \\
    &\ge \|(\bcircA  - \bstAk \bO \bR^{-1})\bR\|_{\fro}^2 + \| (\bcircB - \bstBk \bO \bR^\top)\bR^{-\top}\|_{\fro}^2 \\
    &\ge \sigma_{\min}(\bR)\|\bcircA  - \bstAk \bO\bR^{-1}\|_{\fro}^2 + \sigma_{\min}(\bR^{-\top}) \|\bcircB  - \bstBk \bO \bR^{\top}\|_{\fro}^2 \\
    &\ge \min\{\sigma_{\min}(\bR)^2,\sigma_{\min}(\bR^{-\top})^2\}\|\bcircA  - \bstAk \bO\bR^{-1}\|_{\fro}^2 +  \|(\bcircB  - \bstBk \bO \bR^{\top}\|_{\fro}^2 \\ 
    &\ge ((2-\gamma)\|\bstM\|_{\op}/\gamma\sigma_r(\bstM))^{-1}\left(\|\bcircA  - \bstAk \bO\bR^{-1}\|_{\fro}^2 +  \|\bcircB  - \bstBk \bO \bR^{\top}\|_{\fro}^2\right) \\ 
    \end{align*}
    Thus, 
    \begin{align*}
    \|\bcircA  - \bstAk \bO\bR^{-1}\|_{\fro}^2 +  \|\bcircB  - \bstBk \bO \bR^{\top}\|_{\fro}^2 \le  \epsfro^2 \cdot \frac{(2-\gamma)\cproc\|\bstM\|_{\op}}{\gamma^2\sigma_r(\bstM)^2}. 
    \end{align*}
    \end{proof}
    We can now finish the proof of the lemma. Since $\bV_A \in \R^{r_0 \times r}$ has orthonormal columns, and $r \le r_0$, we have
    \begin{align*}
    \epsfro^2 \cdot \frac{(1+\gamma)\cproc\|\bstM\|_{\op}}{(1-\gamma)^2 \sigma_r(\bstM)^2} 
    & \ge|\bcircA \bV_A^\top  - \bstAk \bO\bR^{-1}\bV_A^\top\|_{\fro}^2 +  \|\bcircB \bV_A^\top - \bstBk \bO \bR^{\top}\bV_A^\top\|_{\fro}^2\\
    &\overset{(i)}{=} \|\btilA  - \underbrace{\bstAk \bO\bR^{-1}\bV_A^\top}_{\bstilAr}\|_{\fro}^2 +  \|\btilB + \bE - \underbrace{\bstBk \bO \bR^{\top}\bV_A^\top}_{\bstilBr}\|_{\fro}^2\\
    \end{align*} 
    where in $(i)$, the term $\bE$ is the error term from \Cref{claim_Eclaim}, and where $\bstilAr := \bstAk \bO\bR^{-1}\bV_A^\top$ and $\bstilBr := \bstBk \bO \bR^{\top}\bV_A^\top$ satisfy $\bstilAr(\bstilBr)^\top =  \bstAk \bO\bR^{-1}\bV_A^\top\bV_A\bR\bO^\top \bstBk = \bstAk(\bstBk)^\top$, where again we use $\bV_A \in \R^{r \times r_0}$ has orthonormal columns and $\bO \in \bbO(r)$. Hence, using \Cref{fact:nice_elementary}
    \begin{align*}
    \epsfro^2 \cdot \frac{(1+\gamma)\cproc\|\bstM\|_{\op}}{(1-\gamma)^2 \sigma_r(\bstM)^2} 
    &\ge \|\btilA  - \bstilAr\|_{\fro}^2 +  \|\btilB + \bE - \bstilBr\|_{\fro}^2
    \ge \|\btilA  - \bstilAr\|_{\fro}^2 +  \frac{1}{2}\|\btilB - \bstilBr\|_{\fro}^2 - \|\bE\|_{\fro}^2\\
    \end{align*}
    Rearranging and invoking the bound on $\|\bE\|_{\fro}^2$ given in \Cref{claim_Eclaim}, we have
    \begin{align*}
    2\|\btilA  - \bstilAr\|_{\fro}^2 +  \|\btilB - \bstilBr\|_{\fro}^2 \le 2\epsfro^2 \cdot \frac{(2-\gamma)\cproc\|\bstM\|_{\op}}{\gamma^2 \sigma_r(\bstM)^2} + 2\trace(\bSigma_B (\bQ \bQ^\top - \eye_{r_0}) \bSigma_B),
    \end{align*}
    
    \end{proof}


\subsubsection{Proof of \Cref{lem:remainder_term}}
    \begin{proof}[Proof of \Cref{lem:remainder_term}]
    Let $\nu \in \R_{< 0}^r$ be given by $\nu_i := \sigma_i(\bhatM)$. Since $\bstPk,\bstQk$ defined in \mscomment{??} are projection operators,
    \begin{align*}
    \max\{\sigma_i(\btilA),\sigma_i(\btilB)\} &= \max\{\sigma_i(\bstPk\bhatA),\sigma_i(\bstQk\bhatB)\}\le \max\{\sigma_i(\bhatA),\sigma_i(\bhatB)\} = \sqrt{\sigma_i(\bhatM)} = \sqrt{\nu_i}. 
    \end{align*} 
    Let $\bSigma_{\nu}$ denote the matrix with diagonals $\nu_i$, so that
    \begin{align*}
    \bSigma_{\nu} \succeq \bSigma_A^2, \quad \bSigma_{\nu} \succeq \bSigma_B^2, \quad \fronorm{\bSigma_{\nu}} = \fronorm{\bhatM_r}
    \end{align*} 
    Hence, 
    \begin{align*}
    \trace(\bSigma_B (\eye_{r_0} - \bQ \bQ^\top ) \bSigma_B) &= \trace(\bSigma_B^2 (\eye_{r_0} - \bQ \bQ^\top ) ) \\
    &\overset{(i)}{\le} \trace(\bSigma_{\nu} (\eye_{r_0} - \bQ \bQ^\top ) )\\
    &\le \frac{1}{\nu_r}\trace(\bSigma_{\nu}^2 (\eye_{r_0} - \bQ \bQ^\top ) )\\
    &= \|\bSigma_{\nu}\|_{\fro}^2 - \trace(\bSigma_{\nu}^2 \bQ \bQ^\top)\\
    &= \|\bSigma_{\nu}\|_{\fro}^2 - \|\bSigma_{\nu}\bQ\|_{\fro}^2.
    \end{align*}
    where in $(i)$ we used $\eye_{r_0} - \bQ \bQ^\top  \succeq 0$ and $\bSigma_B^2 \succeq \bSigma_{\nu}$. Rearranging, 
    \begin{align}
    \|\bSigma_{\nu}\bQ\|_{\fro}^2 \le \|\bSigma_{\nu}\|_{\fro}^2 -  E \label{eq:a_rearrange}
    \end{align}

    Similarly, we compute
     \begin{align*}
    \fronorm{\btilM}^2 &= \fronorm{\bcircA \bcircB^\top}^2  = \fronorm{\bU_A \bSigma_A \bQ \bSigma_B \bU_B^\top}^2\\
    &= \fronorm{\bSigma_A \bQ \bSigma_B }^2 = \trace( \bSigma_B \bQ^\top \bSigma_A^2 \bQ \bSigma_B) = \trace(\bSigma_A^2 \bQ \bSigma^2_B \bQ^\top)\\
    &\le \trace(\bSigma_{\nu} \bQ \bSigma^2_B\bQ^\top) = \trace(\bQ^\top\bSigma_{\nu} \bQ \bSigma^2_B)\\
    &\le \trace(\bQ^\top\bSigma_{\nu} \bQ \bSigma_{\nu}) = \trace(\bQ^\top\bSigma_{\nu} \bQ \bSigma_{\nu})\\
    &\le\fronorm{\bSigma_{\nu}\bQ} \fronorm{\bSigma_{\nu}\bQ^\top}\\
    &\le\fronorm{\bSigma_{\nu}} \fronorm{\bSigma_{\nu}\bQ}
    \end{align*}
    Hence, by \Cref{eq:a_rearrange}
    \begin{align*}
    \fronorm{\btilM}^4 \le \fronorm{\bSigma_{\nu}}^4 - E\fronorm{\bSigma_{\nu}}^2  = \fronorm{\bhatM_r}^4 - \fronorm{\bhatM_r}^2\cdot\trace(\bSigma_B (\eye_{r_0} - \bQ \bQ^\top ) \bSigma_B) 
    \end{align*}
    Therefore, 
    \begin{align*}
    \trace(\bSigma_B (\eye_{r_0} - \bQ \bQ^\top ) \bSigma_B) \cdot \fronorm{\bhatM_r}^2 &\le \fronorm{\bhatM_r}^4 -  \fronorm{\btilM}^4 \\
    &= (\fronorm{\bhatM_r} -  \fronorm{\btilM})(\fronorm{\bhatM_r} +  \fronorm{\btilM})(\fronorm{\bhatM_r}^2 +  \fronorm{\btilM}^2)\\
    &\le4(\fronorm{\bhatM_r} -  \fronorm{\btilM})\max\{\fronorm{\btilM},\fronorm{\bhatM_r}\}^3\\
    &= 4(\fronorm{\bhatM_r} -  \fronorm{\btilM})\fronorm{\bhatM_r}^3,
    \end{align*}
    \mscomment{EXPLAIN STEPS + FIX CONSTANTS}
    Dividing through, 
    \begin{align*}
    \trace(\bSigma_B (\eye_{r_0} - \bQ \bQ^\top ) \bSigma_B) \le 4(\fronorm{\bhatM_r} -  \fronorm{\btilM})\fronorm{\bhatM_r}
    \end{align*}

    To conclude, it suffices to show the following claim:
    \begin{claim} $|\fronorm{\bhatM_r} - \fronorm{\btilM}| \le 2 \epsfro$. 
    \end{claim}
    \begin{proof}
    \begin{align*}
    |\fronorm{\bhatM_r} - \fronorm{\btilM}| &\le |\fronorm{\bhatM_r} - \fronorm{\bstMk}| + |\fronorm{\btilM} - \fronorm{\bstMk}|\\
    &\le |\fronorm{\bhatM_r} - \fronorm{\bstMk}| + |\fronorm{\btilM - \bstMk}|\\
    &\le |\fronorm{\bhatM_r} - \fronorm{\bstMk}| + \epsfro,
    \end{align*}
    where above we used \Cref{eq:norm_equivalence}. Let's finish by bounding $|\fronorm{\bhatM_r} - \fronorm{\bstMk}|$. Recall $\nu_i = \sigma_i(\bhatM_r)$, and set $\nu_i^\star = \sigma_i(\bstMk)$, and let $\nu^\star = (\nu_1^\star,\dots,\nu_r^\star)$ and $\nu = (\nu_1,\dots,\nu_r)$.  Then

    Moreover, we have
    \begin{align*}
    |\fronorm{\bhatM_r} - \fronorm{\bstMk}|^2 &= (\|\nu\| - \|\nu^\star\|)^2\\
    &\le (\|\nu - \nu^\star\|)^2\\
    &= \sum_{i=1}^r (\sigma_i(\bhatM_r) - \sigma_i(\bstMk))^2\\
    &= \sum_{i=1}^r (\sigma_i(\bhatM) - \sigma_i(\bstM))^2 \\
    &\le \sum_{i \ge 1} (\sigma_i(\bhatM) - \sigma_i(\bstM))^2 \\
    &\overset{(i)}{\le} \|\bhatM - \bstM\|_{\fro}^2 = \epsfro^2, 
    \end{align*}
    where in $(i)$ we used \Cref{lem:Mat_pert_one}. 
    \end{proof}
    Applying the above claim to \Cref{eq:second_to_last} concludes. 
    \end{proof}

\subsection{Proof of \Cref{prop:off_projected_factor}}
By orthognality, we have
\begin{align*}
\epsfro^2 = \|\bstM - \bhatM\|_{\fro}^2 &= \fronorm{\bstPk(\bstM - \bhatM)\bstQk}^2 + \fronorm{(\eye_n-\bstPk)(\bstM - \bhatM)\bstQk}^2 \\
&+ \fronorm{\bstPk(\bstM - \bhatM)(\eye_m-\bstQk)}^2 + \fronorm{(\eye_n-\bstPk)(\bstM - \bhatM)(\eye_m-\bstQk)}^2. 
\end{align*}
Thus, lower bound $\fronorm{\bstPk(\bstM - \bhatM)\bstQk}^2 \ge 0$ and using Cauchy Scwhartz,
\begin{align*}
&\fronorm{(\eye_n-\bstPk)(\bstM - \bhatM)\bstQk} + \fronorm{\bstPk(\bstM - \bhatM)(\eye_m-\bstQk)} \\
&\quad+ \fronorm{(\eye_n-\bstPk)(\bstM - \bhatM)(\eye_m-\bstQk)} \le \sqrt{3}\epsfro. 
\end{align*}
In particular, 
\begin{align*}
\fronorm{(\eye_n - \bstPk)(\bstM - \bhatM)} \le \fronorm{(\eye_n - \bstPk)(\bstM - \bhatM) \bstQk} + \fronorm{(\eye_n-\bstPk)(\bstM - \bhatM)(\eye_m-\bstQk)} \le \sqrt{3}\epsfro.
\end{align*}
and similarly, 
\begin{align*}
\fronorm{(\bstM - \bhatM)(\eye_m - \bstQk)} \le \sqrt{3}\epsfro.
\end{align*}
Since $(\eye_n - \bstPk)\bstM = \bstM(\eye_m - \bstQk) = \bstM - \bstMk$, we find
\begin{align*}
\fronorm{(\eye_n - \bstPk)\bhatM} \vee \fronorm{\bhatM(\eye_m - \bstQk)} \le \sqrt{3}\epsfro + \fronorm{\bstM - \bstMk} = \sqrt{3}\epsfro + \tailM(r) 
\end{align*}
To conclude, note that $\fronorm{(\eye_n - \bstPk)\bhatM} = \fronorm{(\eye_n - \bstPk)\bhatA\bhatB^\top} \ge \fronorm{(\eye_n - \bstPk)\bhatM}\sigma_{r_0}(\bhatB)  = \fronorm{(\eye_n - \bstPk)\bhatM}\sigma_{r_0}(\bhatM)^{\half}$ (the inequality follows since $\bhatA,\bhatB$ have inner dimension $r_0$, and equality since $\bhatA,\bhatB$ are balanced). Invoking the similar inequality for $\bhatB$, we find
\begin{align*}
\fronorm{(\eye_n - \bstPk)\bhatM} \vee \fronorm{\bhatM(\eye_m - \bstQk)} \le \frac{\sqrt{3}\epsfro + \tailM(r)}{\sigma_{r_0}(\bhatM)^{\half}}.
\end{align*}
Squaring, and using the elementary inequality $(a+b)^2 \le 2a^2 + 2b^2$, we have
\begin{align*}
\fronorm{(\eye_n - \bstPk)\bhatA}^2 \vee \fronorm{\bhatB(\eye_m - \bstQk)}^2 \le \frac{7\epsfro^2 +  2\tailM^2(r) }{\sigma_{r_0}(\bhatM)}.
\end{align*}





\subsection{}
\newcommand{\bsfR}{\bmsf{R}}
\newcommand{\bsfP}{\bmsf{P}}



\subsection{Proof of \Cref{lem:matdecomp_weighted}}

    Recall that 
    \begin{align*}
    \ErrTerm_0(\bA,\bB) = \|(\bA - \bstAk)(\bstBk)^\top\|_{\fro}^2 \vee \|\bstAk(\bB - \bstBk)^\top\|_{\fro}^2,
    \end{align*}
    where we recall that for some $\bR \in \GL{r_0}$,  $\bA = \bhatA \bR$, and $\bB = \bhatB \R^{-\top}$, so that $\bhatM = \bA\bB^\top$. We bound each term in the sum on the right with its own lemma. Notice that the bounds are symmetric: 
    \begin{lemma}[Key Matrix Error Decomposition]\label{lem:matdecomp_weighted_A} Fix ranks $r,r_1 \in \N$.
    \begin{align*}
    \|(\bA - \bstAk)(\bstBk)^\top\|_{\fro}^2 &\le 10 \max\{1,\|\bR\|_{\op}^2 \} T_1\cdot( \|\bstM\|_{\op} +\|\bstM - \bhatM\|_{\op} ) + 8T_2 + 2T_3,
    \end{align*}
    where we define the error terms
    \begin{align}
    T_1 &:= \|\bstPk\bhatP_{r_1}\bA - \bstAk\|_{\fro}^2 + \|\bstQk\bhatQ_{r_1}\bB - \bstBk\|_{\fro}^2 \label{eq:T_one_app}\\
    T_2&:= \|\bhatM_{>r_1}\|_{\fro}^2\label{eq:T_two_app}\\
    T_{3,A} &:= \|(\eye_n-\bstPk)\bhatM\|_{\fro}^2\label{eq:T_three_A_app}. 
    \end{align}
    \end{lemma}
    The proof of the above lemma is provided below. 
    The analogous bound to control $\bB - \bstBk$ is given as follows.
    \begin{lemma}\label{lem:matdecomp_weighted_B}
    Similarly to \Cref{lem:matdecomp_weighted_A}, we have
    \begin{align*}
    \|\bstAk(\bB - \bstBk)^\top\|_{\fro}^2 &\le 10\max\{1,\|\bR^{-1}\|_{\op}^2 \}T_1\cdot( \|\bstM\|_{\op} +\|\bstM - \bhatM\|_{\op} ) + 8T_2 + 2T_{3,B},
    \end{align*}
    where $T_1$ and $T_2$ are as in \Cref{lem:matdecomp_weighted_A}, and where $T_{3,B} := \|\bhatM(\eye_m-\bstQk)\|_{\fro}^2$. 
    \end{lemma}
    Due to its similarity to \Cref{lem:matdecomp_weighted_A}, the proof of \Cref{lem:matdecomp_weighted_B} is ommitted. Adding the two bounds yields
    \begin{multline*}
    \|(\bA - \bstAk)(\bstBk)^\top\|_{\fro}^2 \vee \|\bstAk(\bB - \bstBk)^\top\|_{\fro}^2  \le \\
    10\max\{1,\|\bR\|_{\op}^2,\|\bR^{-1}\|_{\op}^2\} T_1\cdot( \|\bstM\|_{\op} +\|\bstM - \bhatM\|_{\op} ) + 8T_2 + 2T_3,
    \end{multline*}
    where
    \begin{align*}
    T_{3} &:= T_{3,A} \vee T_{3,B}  = \|(\eye_n-\bstPk)\bhatM\|_{\fro}^2 \vee \|\bhatM(\eye_m-\bstQk)\|_{\fro}^2.
    \end{align*}
    Noting $\max\{1,\|\bR\|_{\op}^2,\|\bR^{-1}\|_{\op}^2\} = \max\{\|\bR\|_{\op}^2,\|\bR^{-1}\|_{\op}^2\} = \mu(\bR)^2$ (as $\max\{\|\bR\|_{\op},\|\bR^{-1}\|_{\op}\}\ge 1$) concludes the proof of \Cref{lem:matdecomp_weighted}.\qed
    \linebreak
    \begin{proof}[Proof of \Cref{lem:matdecomp_weighted_A}]
    \begin{align*}
    &\|(\bA - \bstAk)(\bstBk)^\top\|_{\fro}^2\\
     &= \|\bstPk(\bA - \bstAk)(\bstBk)^\top\|_{\fro}^2 + \|(\eye_n-\bstPk)(\bA - \bstAk)(\bstBk)^\top\|_{\fro}^2 \tag{$\bstPk$ is a projection} \\
    &= \|\bstPk(\bA - \bstAk)(\bstBk)^\top\|_{\fro}^2 + \|(\eye_n-\bstPk)\bA(\bstBk)^\top\|_{\fro}^2 \tag{$\bstPk \bstAk = \bstAk$} \\
    &= \|\bstPk(\bA - \bstAk)(\bstBk)^\top\|_{\fro}^2 + \|(\eye_n-\bstPk)\bA(\bstBk)^\top\bstQk\|_{\fro}^2 \tag{$\bstQk \bstBk = \bstBk$}\\
    &= \|\bstPk(\bA - \bstAk)(\bstBk)^\top\|_{\fro}^2 + \|(\eye_n-\bstPk)\left(\bA\bB^\top-\bA(\bB - \bstBk)^\top \right)\bstQk\|_{\fro}^2\\
    &\le \|\bstPk(\bA - \bstAk)(\bstBk)^\top\|_{\fro}^2 + 2\|(\eye_n-\bstPk)\bA\bB^\top\bstQk\|_{\fro}^2 + 2\|(\eye_n-\bstPk)\bA(\bB - \bstBk)^\top \bstQk\|_{\fro}^2\\
    &= \|(\bstPk\bA - \bstAk)(\bstBk)^\top\|_{\fro}^2 + 2\|(\eye_n-\bstPk)\bA\bB^\top\bstQk\|_{\fro}^2 + 2\|(\eye_n-\bstPk)\bA(\bstQk\bB - \bstBk)^\top \|_{\fro}^2\\
    &\le \|(\bstPk\bA - \bstAk)(\bstBk)^\top\|_{\fro}^2 + 2\|(\eye_n-\bstPk)\bA\bB^\top\|_{\fro}^2 + 2\|(\eye_n-\bstPk)\bA(\bstQk\bB - \bstBk)^\top \|_{\fro}^2,
    \end{align*}
    where in the last two lines we use $\bstQk \bstBk = \bstBk$, followed by the fact that $\bstQk$ is a projection. 


    We further split
    \begin{align*}
    &\|(\bstPk\bA - \bstAk)(\bstBk)^\top\|_{\fro}^2 \\
    &\le 2\|(\bstPk\bhatP_{r_1}\bA - \bstAk)(\bstBk)^\top\|_{\fro}^2 + 2\|\bstPk(\eye - \bhatP_{r_1})\bA (\bstBk)^\top\|_{\fro}^2 \\
    &\le 2\|(\bstPk\bhatP_{r_1}\bA - \bstAk)(\bstBk)^\top\|_{\fro}^2 \\
    &\qquad+ 4\|(\bstPk(\eye - \bhatP_{r_1})\bA (\bstBk - \bstQk \bhatQ_{r_1}\bB)^\top\|_{\fro}^2 +  4\|\bstPk(\eye - \bhatP_{r_1})\bA (\bstQk \bhatQ_{r_1}\bB)^\top\|_{\fro}^2 \\
    &\le 2\|\bstBk\|_{\op}^2\|\bstPk\bhatP_{r_1}\bA - \bstAk\|_{\fro}^2 \tag{$\bstQk$, $\bhatQ_{r_1}$ are projections, see the last term}\\
    &\qquad + 4\|\bstPk(\eye - \bhatP_{r_1})\bA\|_{\op}^2 \|\bstBk -  \bstQk \bhatQ_{r_1}\bB\|_{\fro}^2 +  4\|\bstPk(\eye - \bhatP_{r_1})\bA \bB^\top\|_{\fro}^2 \\
    &\overset{(i)}{\le} 2\|\bstM\|_{\op}\|\bstPk\bhatP_{r_1}\bA - \bstAk\|_{\fro}^2 + 4\|\bR\|^2_{\op}\opnorm{\bhatM}\|\bstBk -  \bstQk \bhatQ_{r_1}\bB\|_{\fro}^2 +  4\|\bstPk(\eye - \bhatP_{r_1})\bA \bB^\top\|_{\fro}^2\\
    &= 2\|\bstM\|_{\op}\|\bstPk\bhatP_{r_1}\bA - \bstAk\|_{\fro}^2 + 4\|\bR\|^2_{\op}\opnorm{\bhatM}\|\bstBk -  \bstQk \bhatQ_{r_1}\bB\|_{\fro}^2 +  4\|\bstPk \bhatM_{>r_1}\|_{\fro}^2. 
    \end{align*}
    where in $(i)$ we use that $\|\bstBk\|_{\op} \le \|\bstB\|_{\op}$, and $(\bstA,\bstB)$ is a balanced of $\bstM$, and use $\|\bstPk(\eye - \bhatP_{r_1})\bA\|_{\op}^2 \le \|\bA\|_{\op}^2 = \|\bhatA\bR\|_{\op}^2 \le \|\bR\|^2_{\op}\|\bhatA\|_{\op}^2$, again using that $(\bhatA,\bhatB)$ is balanced (though this latter bound is crude, refining it only improves constant factors at the end). 
    Similarly, 
    \begin{align*}
    &2\|(\eye_n-\bstPk)\bA(\bstQk\bB - \bstBk)^\top \|_{\fro}^2 \\
    &\le 4\|(\eye_n-\bstPk)\bA(\bstQk\bhatQ_{r_1}\bB - \bstBk)^\top \|_{\fro}^2 + 4\|(\eye_n-\bstPk)\bA(\bstQk(\eye_m-\bhatQ_{r_1})\bB)^\top  \|_{\fro}^2\\
    &\le 4\|(\eye_n-\bstPk)\bA\|_{\op}^2 \|\bstQk\bhatQ_{r_1}\bB - \bstBk \|_{\fro}^2 + 4\|\bA(\bstQk(\eye_m-\bhatQ_{r_1})\bB)^\top \|_{\fro}^2\\
    &= 4\|(\eye_n-\bstPk)\bA\|_{\op}^2 \|\bstQk\bhatQ_{r_1}\bB - \bstBk \|_{\fro}^2 + 4\|\bA\bB^\top (\eye_m - \bhatQ_{r_1})\bstQk\|_{\fro}^2\\
    &= 4\|(\eye_n-\bstPk)\bA\|_{\op}^2 \|\bstQk\bhatQ_{r_1}\bB - \bstBk \|_{\fro}^2 + 4\|\bhatM_{> r_1} \bstQk\|_{\fro}^2\\
    &\le 4\|\bR\|_{\op}^2\|\bhatM\|_{\op} \|\bstQk\bhatQ_{r_1}\bB - \bstBk\|_{\fro}^2 + 4\|\bhatM_{> r_1} \bstQk\|_{\fro}^2
    \end{align*}
    where in the last line, we use $\|(\eye_n-\bstPk)\bA\|_{\op}^2 \le \|\bA\|_{\op}^2  \le \|\bR\|_{\op}^2 \|\bhatM\|_{\op}$, as above.  Thus, all in all, we bound
    and 
    \begin{align*}
    &\|(\bA - \bstAk)(\bstBk)^\top\|_{\fro}^2 \\
    &\le 2\|\bstM\|_{\op}\|\bstPk\bhatP_{r_1}\bA - \bstAk\|_{\fro}^2 +  8\|\bR\|_{\op}^2\|\bhatM\|_{\op}  \|\bstQk\bhatQ_{r_1}\bB - \bstBk\|_{\fro}^2 \\
    &\quad+ 4\underbrace{\left(\|\bstPk \bhatM_{>r_1}\|_{\fro}^2+ \|\bhatM_{> r_1} \bstQk\|_{\fro}^2\right)}_{\le 2\|\bhatM_{>r_1}\|_{\fro}^2 = 2T_2} + 2\underbrace{\|(\eye_n-\bstPk)\bA\bB^\top\|_{\fro}^2}_{T_3,A}
    \end{align*}
    To conclude, we see the term on the first line is at most
    \begin{align*}
    10\max\{1,\|\bR\|_{\op}^2\}(\|\bstM - \bhatM\|_{\op} + \|\bstM\|_{\op})\left(\underbrace{\|\bstPk\bhatP_{r_1}\bA - \bstAk\|_{\fro}^2 + \|\bstQk\bhatQ_{r_1}\bB - \bstBk\|_{\fro}^2}_{T_1}\right)
    \end{align*}
    \end{proof}


\subsection{Bounding terms $T_2$ and $T_3$ \label{app:t2_t3}}
    
    
    \begin{proof}[Proof of \Cref{lem:t2_bound}] Using  the elementary inequality $a^2 \le 2(a-b)^2 + 2b^2$, we have
    \begin{align*}
    T_2(r_1) &= \|\bhatM_{>r_1}\|_{\fro}^2 = \sum_{i=r_1+1}^{r}\sigma_i(\bhatM)^2\\
    &\le  2\sum_{i=r_1+1}^{r}(\sigma_i(\bhatM)-\sigma_i(\bstM))^2 + 2\sum_{i=r_1+1}^{r}\sigma_i(\bstM)^2\\
    &\le  2\|\bhatM - \bstM\|_{\fro}^2 + 2\sum_{i=r_1+1}^{r}\sigma_i(\bstM)^2 =  2\epsfro^2 + 2\epsapx(r_1),
    \end{align*}
    where in the last line, we used \Cref{lem:Mat_pert_one}. 
    \end{proof}
    \begin{proof}[Proof of \Cref{lem:t3_bound}]  SInce $(\eye_n-\bstPk)\bstMk = \bstMk(\eye_m-\bstQk) = 0$, we have
    \begin{align*}
    \|(\eye_n-\bstPk)\bhatM\|_{\fro}^2 \vee  \|\bhatM(\eye_m-\bstQk)\|_{\fro}^2 &= \|(\eye_n-\bstPk)(\bhatM - \bstMk)\|_{\fro}^2 \vee  \|(\bstMk - \bhatM)(\eye_m-\bstQk)\|_{\fro}^2\\
    &\le  \|\bhatM - \bstMk\|_{\fro}^2 \\
    &\le  2\|\bhatM - \bstM\|_{\fro}^2 + 2\|\bstM - \bstMk\|_{\fro}^2\\
    &\le 2\epsfro^2 + 2\epsapx(k).
    \end{align*}
    \end{proof}


\subsection{Application of Wedin}

    \begin{lemma}[Singular Value Approximation]\label{lem:ssv_approx} Let $\bhatM,\bstM \in \R^{m \times n}$ be two matrices. Fix a $\tau > 0$, and let $r_1,k \in \N$, and let $(1-\tau)\sigma_k(\bstM) \ge \sigma_{r_1+1}(\bhatM)$. Then, if $\bstPk,\bstQk$ denote the projections onto the top $r$ left (resp. right) singular vectors of $\bstM$, then
    \begin{align*}
    \|\bstPk\left(\bhatM_{r_1} - \bstM\right)\bstQk\|_{\fro} = \|\bstPk\bhatM_{r_1}\bstQk - \bstMk\|_{\fro} \le \left(1+ \frac{2}{\tau}\right)\|\bhatM - \bstM\|_{\fro}.
    \end{align*}
    where we let $\bhatM_{r_1}$ denote the rank $r_1$-SVD of $\bhatM$, and $\bstMk$ the rank $r$-SVD of $\bstM$. In addition, the same holds with Frobenius norm replaced by the operator norm. 
    \end{lemma}
    \begin{proof} We may assume $\sigma_{r_1+1}(\bhatM) > 0$, for otherwise $\bhatM_{r_1} = \bhatM$ and the bound is straightforward. 

    Let $\circnorm{\cdot}$ denote Frobenius or operator norm. Set $\epsilon = \|\bhatM - \bstM\|_{\circ}$, and decompose $\bhatM$ into $\bhatM_{r_1} + \bhatM_{< r_1}$, where $\bhatM_{< r_1}$ contains singular values of $\bhatM$ which are $< \sigma_{r_1}(\bhatM)$. We then have
    \begin{align*}
    \|\bstPk\left(\bhatM_{r_1} - \bstM\right)\bstQk\|_{\circ} &= \|\bstPk\left((\bhatM - \bhatM_{< r_1}) - \bstM\right)\bstQk\|_{\circ}\\
    &\le \|\bstPk\left(\bhatM - \bstM\right)\bstQk\|_{\circ} + \|\bstPk\bhatM_{< r_1}\bstQk\|_{\circ}\\
    &\le \epsilon + \|\bstPk\bhatM_{< r_1}\bstQk\|_{\circ},
    \end{align*}
    where in the last step, we used that $\bstPk,\bstQk$ are projection matrices. 

    To finish, it suffices to prove $\|\bstPk\bhatM_{< r_1}\bstQk\|_{\circ} \le \frac{2\epsilon}{\tau}$. To this end,  $\bhatM_{> r_1} = \bhatU_{< r_1} \bhatSigma_{< r_1} \bhatV_{< r_1}^\top$ and $\bstMk = \bstUk \bstSigma_r (\bstVk)^\top$. Since $\bstPk = \bstUk(\bstUk)^\top$ and $\bstQ_R = \bstVk(\bstVk)^\top$, we can use $\|\bstUk\|_{\op} = \|\bstVk\|_{\op} = \|\bhatV_{<r_1}\|_{\op} = 1$ to crudely bound
    \begin{align*}
    \|\bstPk\bhatM_{< r_1}\bstQk\|_{\circ} &= \|\bstUk(\bstUk)^\top\bhatU_{< r_1} \bhatSigma_{< r_1} \bhatV_{< r_1}^\top\bstVk(\bstVk)^\top\|_{\circ}\\
    &\le \|(\bstUk)^\top\bhatU_{< r_1} \bhatSigma_{< r_1}\|_{\circ}\\
    &\le \|(\bstUk)^\top\bhatU_{< r_1}\|_{\circ} \|\bhatSigma_{< r_1}\|_{\op}\\
    &= \|(\bstUk)^\top\bhatU_{< r_1}\|_{\circ}\cdot \sigma_{r_1+1}(\bhatM). 
    \end{align*}
    Since $\bstUk$ corresponds to the singular space of $\bstMk$ with singular values $\ge \sigma_k(\bstM)$, and $\bhatU_{< r_1}$ corresponds to singular values  $\le (1-\tau) \sigma_k(\bstM) $, \Cref{lem:gap_free_Wedin} implies that
    \begin{align*}
    \|(\bstUk)^\top\bhatU_{< r_1}\|_{\circ} \le \|(\bstUk)^\top\bhatU_{\le r_1}\|_{\circ} \le \frac{2\circnorm{\bhatM - \bstM}}{\tau \sigma_k(\bstM)} \le \frac{2\epsilon}{\tau \sigma_{r_1+1}(\bhatM)},
    \end{align*}
    where above we use $\sigma_k(\bstM) \ge \sigma_{r_1+1}(\bhatM)$.
    Hence, by the previous display, we conclude $\|\bstPk\bhatM_{< r_1}\bstQk\|_{\circ} \le \frac{2\epsilon}{\tau}$, as needed. 
    \end{proof}

    \begin{lemma}\label{lem:proj_lowner}Consider the set up of \Cref{lem:ssv_approx}, where for some $\tau \in (0,1)$, $(1-\tau)\sigma_k(\bstM) \ge \sigma_{r_1+1}(\bhatM)$. Then,
    \begin{align*}
    (\bstPk \bhatA_{k})^\top (\bstPk \bhatA_{k})\succeq f(\tau)\bhatA_k^\top \bhatA_k, \quad (\bstQk \bhatB_{k})^\top (\bstQk \bhatB_{k}) \succeq f(\tau)\bhatB_k^\top \bhatB_k,
    \end{align*} 
    where $f(\tau) := 1 - \frac{4\|\bstM - \bhatM_{\op}\|}{\tau \sigma_k(\bstM)}$. 
    \end{lemma}
    \begin{proof}
    We prove the bound of $\bhatA$, as the corresponding bound of $\bhatB$ is analougs. Let $\bstU_k$, and $\bhatU_k$ denote the basis for the top $k$ left singular vectors of $\bstM$ and $\bhatM$, respectively. Note that these correspond to the top-$k$ left singular vectors of $\bstA$ and $\bhatA$, respectively, as well. Let $\bstP_k = \bstU_k(\bstU_k)^\top$, $\bhatP_k = \bhatU\bhatU_k^\top$, and define $\bstP_{> k}$, $\bhatP_{>k}$, $\bstU_{>k}$ and $\bhatU_{>k}$ as the corresponding projections and bases for singular vectors for singular values $i > k$.

     Since $\bhatA_{k} = \bU_{k}\bU_{k}^\top\bhatA_{k}$, we then have 
    \begin{align*}
    \bstPk \bhatA_{k}= \bstPk  \bhatP_k\bhatA_{k}
    \end{align*}
    Therefore, 
    \begin{align*}
    (\bstPk \bhatA_{k})^\top (\bstPk \bhatA_{k}) &= \bhatA_{k}^\top (\bstP_k \bhatP_k)^\top (\bstP_k \bhatP_k)\bhatA_{k}^\top\\
    &\succeq \bhatA_{k}^\top (\bhatP_k \bstP_k \bhatP_k) \bhatA_{k}^\top\\
    &\succeq \sigma_{k}(\bhatP_k \bstP_k \bhatP_k) \bhatA_{k}^\top\bhatA_{k},
    \end{align*}
    where in the last inequality, we used that $\range(\bhatA_k) = (\bhatP_k \bstP_k \bhatP_k)$.  By Weyl's ienquality,
    \begin{align*}
    \sigma_{k}(\bhatP_k \bstP_k \bhatP_k) &\ge  \sigma_k(\bstP_k) - \|\bstP_k - \bhatP_k \bstP_k \bhatP_k\|_{\op} \\
    &=  1 - \|\bstP_k - \bhatP_k \bstP_k \bhatP_k\|_{\op} \\
    &\ge  1 - (\|(\eye_n - \bhatP_k)\bstP_k\|_{\op} + \|\bhatP_k \bstP_k (\eye_n - \bhatP_k)\|) \\
    &\ge  1 -(\|(\eye_n - \bhatP_k)\bstP_k\|_{\op} + \| \bstP_k (\eye_n - \bhatP_k)\|_{\op}) \\
    &=  1 - (\|\bhatP_{>k}\bstP_k\|_{\op} + \| \bstP_k \bhatP_{>k}\|_{\op}) \\
    &=  1 - (\|\bhatU_{>k}\bhatU_{>k}^\top \bstU_k (\bstU_k)^\top\|_{\op} + \| \bstU_k (\bstU_k)^\top\bhatU_{>k}(\bhatU_{>k})^\top\|_{\op}) \\
    &\ge  1 - (\|\bhatU_{>k}^\top \bstU_k\|_{\op} + \|(\bstU_k)^\top\bstU_{>k} \|) \\
    &=  1 - 2\|(\bstU_k)^\top\bhatU_{>k}\|_{\op}.
    \end{align*}
    By applying the operator-norm statement of \Cref{lem:gap_free_Wedin} with $\tau \gets \tau \cdot \sigma_{k}(\bstM)$, we have 
    \begin{align*}
    \|(\bstU_k)^\top\bhatU_{>k}\|_{\op}  \le \frac{2\|\bstM - \bhatM_{\op}\|}{\tau \sigma_k(\bstM)}. 
    \end{align*}
    Hence, 
    \begin{align*}
    \sigma_{k}(\bhatP_k \bstP_k \bhatP_k) \ge 1 -  \frac{4\|\bstM - \bhatM_{\op}\|}{\tau \sigma_k(\bstM)} =: f(\tau). 
    \end{align*}
    The bound follows. 
    \end{proof}

   
    \wedinapply*
    \begin{proof} We first verify $\sigma_k(\bstM) \ge (1+\tau)\sigma_{k+1}(\bhatM)$ for some $\tau = 5\delstk/6$. From Weyl's inequalities, we have
    \begin{align*}
    \sigma_{k+1}(\bhatM) &\le \|\bhatM - \bstM\|_{\op} + \sigma_{k+1}(\bstM) \\
    &\le \|\bhatM - \bstM\|_{\op} + \sigma_{k+1}(\bstM) \\
    &= \sigma_{k}(\bstM)\left(\frac{\|\bhatM - \bstM\|_{\op}}{\sigma_{k}(\bstM) } + \frac{\sigma_{k+1}(\bstM)}{\sigma_k(\bstM)}\right)\\
    &= \sigma_{k}(\bstM)\left(1 + \frac{\|\bhatM - \bstM\|_{\op}}{\sigma_{k}(\bstM) } -\delstk\right)
    \end{align*}
    In particular, if $\frac{\|\bhatM - \bstM\|_{\op}}{\sigma_{k}(\bstM) } \le \delstk/6$, then
    \begin{align}
    \sigma_{k+1}(\bhatM) \le (1-\tau) \sigma_{k}(\bstM), \quad \tau = 5\delstk/6 \label{eq:tau_bound}.
    \end{align}
    \textbf{Item (a).} Hence, \Cref{lem:ssv_approx} and using $\delstk \le 1$ gives 
    \begin{align*}
    \|\bstPk\bhatM_{k}\bstQk - \bstMk\|_{\fro} \le \left(1+ \frac{12}{5\delstk}\right)\|\bhatM - \bstM\|_{\fro} \le \frac{17}{5\delstk}\|\bhatM - \bstM\|_{\fro} \le \frac{4}{\delstk}\|\bhatM - \bstM\|_{\fro}. 
    \end{align*}
    \textbf{Item (b).} Similarly, using the operator norm variant of \Cref{lem:ssv_approx}, togegether with $\frac{\|\bhatM - \bstM\|_{\op}}{\sigma_{k}(\bstM) } \le \delstk/6$ gives
    \begin{align*}
    \|\bstPk\bhatM_{k}\bstQk - \bstMk\|_{\op}  \le \frac{17}{5\delstk}\|\bhatM - \bstM\|_{\op} \le \frac{4}{\delstk}\|\bhatM - \bstM\|_{\op} \le \frac{2}{3}\sigma_{k}(\bstM).
    \end{align*}
    \textbf{Item c.} Finally, using \Cref{lem:proj_lowner} with $f(\tau) = 1 - \frac{4\|\bstM - \bhatM_{\op}\|}{\tau \sigma_k(\bstM)} = 1 - \frac{4\delstk}{6\tau} = 1 - \frac{4\delstk}{6}\cdot \frac{6}{5\delstk} = \frac{1}{5}$, we conclude:
    \begin{align*}
    (\bstPk \bhatA_{k})^\top (\bstPk \bhatA_{k}) \succeq \frac{1}{5}\bhatA_k^\top \bhatA_k, \quad (\bstQk \bhatB_{k})^\top (\bstQk \bhatB_{k}) \succeq \frac{1}{5}\bhatB_k^\top \bhatB_k.
    \end{align*}
    To check the rank condition, we see lower bound 
    \begin{align*}
    k \ge \min\{\rank(\bstPk \bhatA_{k}),\rank(\bstQk \bhatB_{k})\} \ge \rank(\bstPk\bhatA_k(\bstQ_k\bhatB_k)^\top) = \rank(\bstPk\bhatM_k\bstQk),
    \end{align*}
    where above we used $\bhatA_k\bhatB_k^\top = \bhatM$ and $\bstQk = (\bstQk)^\top$.  Item $(b)$ together with Weyl's inequality entails $\sigma_k(\bstPk\bhatM_k\bstQk) \ge \sigma_k(\bstM_k) - \frac{2}{3}\sigma_k(\bstM) = \sigma_k(\bstM)/3 > 0$, so that $\rank(\bstPk\bhatM_k\bstQk) \ge k$. 

    \end{proof}

    \lemtilbalance*
    
    \begin{proof} For simplicity, let $\bbarA_k = \bstP_k\bhatA_k$ and $\bbarB_k := \bstQ_k \bhatB_k$. Since $\bbarA_k$ and $\bbarB_k$ are both rank $r$ (\Cref{lem:wedin_closeness_aplied}), \mscomment{..} implies that there exists a matrix $\bW \succ 0$ such that
    \begin{align*}
    \bW \bbarA_k^\top \bbarA_k \bW = (\bbarB_k^\top \bbarB_k).
    \end{align*}

    By \Cref{lem:wedin_closeness_aplied} part (c), we find
    \begin{align*}
    \bbarB_k^\top \bbarB_k &\succeq \frac{1}{5}\bhatB_k^\top \bhatB_k \tag{\Cref{lem:wedin_closeness_aplied}, part (c)}\\
    &=\frac{1}{5}\bhatA_k^\top \bhatA_k \tag{$\bhatA_k$, $\bhatB_k$ is balanced. } \\
    &\succeq \frac{1}{5}\bhatA_k^\top \bstP_k \bhatA_k  \tag{$\bstP_k \preceq \eye_n$}\\
    &=  \frac{1}{5}(\bstP_k\bhatA_k)^\top (\bstP_k \bhatA_k) \tag{$\bstP_k $ is a projection}\\
    &=  \frac{1}{5}\bbarA_k^\top \bbarA_k.  %, \quad \bbarB_k^\top \bbarB_k \succeq \frac{1}{5}\bhatA_B^\top \bhatB_k,
    \end{align*}
    Similarly, $\bbarA_k^\top \bbarA_k \succeq \frac{1}{5}\bbarB_k^\top \bbarB_k$. Hence, by \Cref{lem:bal_properties}, part (d),
    \begin{align*}
    5^{-1/2}\eye_k \preceq \bW \preceq \eye_k 5^{1/2}.
    \end{align*}
    Writing $\bW = \bR\bR^\top$ (this decomposition exists such $\bW \succ 0$), and notince $\max\{\|\bR\|_\op,\|\bR^{-1}\|_{\op}\}^2 \le \sqrt{5}$,
    \begin{align*}
    \bR\bR^\top\bbarA_k^\top \bbarA_k \bR\bR^{\top} = \bbarB_k^\top \bbarB_k &\iff \bR^\top\bbarA_k^\top \bbarA_k \bR = \bR^{-1}\bbarB_k^\top \bbarB_k\bR^{-\top}\\
    &\iff (\bbarA_k \bR)^\top (\bbarA_k \bR) = (\bbarB_k \bR^{-\top})^\top(\bbarB_k \bR^{-\top}).
    \end{align*}
    Hence, $\btilA_k := \bbarA_k \bR$ and $\btilB_k := \bbarB_k \bR^{-\top}$ satisfy the conclusion of the theorem. 
    \end{proof}


\subsection{Proof of \Cref{lem:projection_conditioning}}
We begin with a few technical lemmas
\begin{lemma}\label{lem:von_neuman_one} Let $\bM = \bA \bB^\top$ have rank (at most) $r$. Then, $\sum_{i=1}^r \sigma_i(\bM) \le \sum_{i=1}^r \sigma_i(\bA)  \sigma_i(\bB)$. 
\end{lemma}

\begin{lemma}\label{lem:von_neuman_sq} Let $\bM = \bA \bB^\top$ have rank (at most) $r$. 
 $\sum_{i=1}^r \sigma_i(\bM)^2 \le \sum_{i=1}^r \sigma_i(\bA)^2  \sigma_i(\bB)^2$. As a consequence, $\|\bM\|_{\fro} \le \|\bSigma_A\bSigma_B\|_{\fro}$, where $\bSigma_A,\bSigma_B$ contain the singular values of $\bA,\bB$ in non-decreasing order. 
\end{lemma}

\begin{lemma}\label{lem:Mat_pert_one} For any $\bM,\bM' \in \R^{m \times n}$,
\begin{align*}
\sum_{i=1}^{\nu} (\sigma_i(\bM)-\sigma_i(\bM'))^2 \le \|\bM - \bM'\|_{\fro},
\end{align*}
where the above holds for $\nu = \min(n,m)$, and thus, also holds for any $1 \le \nu \le \min(n,m)$. 
\end{lemma}
\begin{comment}

\begin{claim}
\begin{align*}
\|\bstM - \bhatM\|_{\fro}^2 \ge  \max\left\{\sum_{i=1}^{r} |\sigma_i(\bstM) - \sigma_i(\btilM)|^2, \sum_{i=1}^{r} |\sigma_i(\bstM) - \sigma_i(\bhatM)|^2\right\}
\end{align*}
Thus, by an application of the triangle inequality, 
\begin{align*}
\sum_{i=1}^{r} |\sigma_i(\btilM)|^2 \ge    \sum_{i=1}^{r} |\sigma_i(\bhatM)|^2 - 4 \|\bstM - \bhatM\|_{\fro} \sqrt{\sum_{i=1}^{r} |\sigma_i(\bhatM)|^2}
\end{align*}
\end{claim}
\begin{proof}The inequality involving $\bhatM$ follows directly from \Cref{lem:Mat_pert_one}. Applying that same lemma, we also find
\begin{align*}
\sum_{i=1}^{r} |\sigma_i(\underbrace{\bstP_r\bstM\bstQ_r}_{\btilM}) - \sigma_i(\bstP_r\bhatM\bstQ_r)|^2 \le \|\bstP_r(\bstM - \bhatM)\bstQ_r\|_{\fro}^2 \le   \|\bstM - \bhatM\|_{\fro}^2. 
\end{align*}
Hence, by applying the triangle inequality to the vectors $(\sigma_i(\btilM))$, $(\sigma_i(\bhatM))$, $(\sigma_i(\bstM))$,
\begin{align*}
\sqrt{\sum_{i=1}^{r} |\sigma_i(\btilM) - \sigma_i(\bhatM)|^2} \le  2 \|\bstM - \bhatM\|_{\fro}.
\end{align*}
Another application of the triangle inequality yields. 
\begin{align*}
\sqrt{\sum_{i=1}^{r} |\sigma_i(\btilM)|^2} \ge  - 2 \|\bstM - \bhatM\|_{\fro} + \sqrt{\sum_{i=1}^{r} |\sigma_i(\bhatM)|^2}.
\end{align*}
Squaring gives
\begin{align*}
\sum_{i=1}^{r} |\sigma_i(\btilM)|^2 \ge    \sum_{i=1}^{r} |\sigma_i(\bhatM)|^2 - 4 \|\bstM - \bhatM\|_{\fro} \sqrt{\sum_{i=1}^{r} |\sigma_i(\bhatM)|^2}
\end{align*}
\end{proof}

\begin{claim} Suppose that $\alpha_r := \left(1 - 4 \frac{\|\bstM - \bhatM\|_{\fro}\|\bhatM\|_{\fro}}{\sigma_r(\bhatM)^2}\right) > 0$. Then, we have that
\begin{align*}
\alpha_{r} \le \frac{\sigma_j(\bstQ_r \bhatB)^2}{\sigma_j(\bstQ_r \bhatA)^2}  \le \alpha_r^{-1}, \quad \forall j \in [r],
\end{align*}
\end{claim}
\begin{proof}
For any $j \in [r]$, we find
\begin{align*}
\sum_{i=1}^r \sigma_i(\btilM)^2 &\le \sum_{i=1}^r\sigma_i(\bstP_r \bhatA)^2\sigma_i(\bstQ_r \bhatB)^2 \\
&\le \sum_{i=1, i \ne j}^r \sigma_i(\bhatA)^2\sigma_i(\bhatB)^2 + \sigma_j(\bstP_r \bhatA)^2\sigma_j(\bstQ_r \bhatB)^2\\
&\le \sum_{i=1, i \ne j}^r \sigma_i(\bhatA)^2\sigma_i(\bhatB)^2 + \sigma_j(\bstP_r \bhatA)^2\sigma_j(\bhatB)^2\\
&= \sum_{i=1, i \ne j}^r \sigma_i(\bhatM)^2 + \sigma_j(\bstP_r \bhatA)^2\sigma_j(\bhatM).
\end{align*}
Applying the above claim and cancelling terms $i \ne j$ gives
\begin{align*}
\sigma_j(\bhatM)^2 - 4 \|\bstM - \bhatM\|_{\fro} \underbrace{\sqrt{\sum_{i=1}^{r} |\sigma_i(\bhatM)|^2}}\le \sigma_j(\bstP_r \bhatA)^2\sigma_j(\bhatM), \quad \forall r\in [j]
\end{align*}
Dividing by $\sigma_j(\bhatM)$ and factoring the left hand side yields, and lower bounding $\sqrt{\sum_{i=1}^{r} |\sigma_i(\bhatM)|^2} \le \|\bhatM\|_{\fro}$ yields
\begin{align*}
\sigma_j(\bhatM) \left(1 - 4 \frac{\|\bstM - \bhatM\|_{\fro}\|\bhatM\|_{\fro}}{\sigma_j(\bhatM)^2}\right)  \le \sigma_j(\bstP_r \bhatA)^2,\quad \forall r \in [j]
\end{align*}
Finally, lower bounding $ \sigma_j(\bhatM) \ge \sigma_r(\bhatM)$  for $j \in [r]$, and noting $\sigma_j(\bstP_r \bhatA)^2 \le \sigma_j(\bhatA)^2 = \sigma_j(\bhatM)$, we conclude, 
\begin{align*}
\sigma_j(\bhatM) \underbrace{\left(1 - 4 \frac{\|\bstM - \bhatM\|_{\fro}\|\bhatM\|_{\fro}}{\sigma_r(\bhatM)^2}\right)}_{:= \alpha_r}  \le  \sigma_j(\bstP_r \bhatA)^2 \le \sigma_j(\bhatM),\quad \forall r \in [j]
\end{align*}
A symmetric argument reveals 
\begin{align*}
\sigma_j(\bhatM) \alpha_r \le  \sigma_j(\bstQ_r \bhatB)^2 \le \sigma_j(\bhatM),\quad \forall r \in [j]
\end{align*}
By considering the ratios of the above inequalities and using $\alpha_r < 1$, we have that (for $\alpha_r > 0$),
\begin{align*}
\alpha_{r} \le \frac{\sigma_j(\bstQ_r \bhatB)^2}{\sigma_j(\bstQ_r \bhatA)^2}  \le \alpha_r^{-1}, \quad \forall j \in [r],
\end{align*}
concluding the proof of the claim. 
\end{proof}
The proof of \Cref{lem:projection_conditioning} follows from the previous claim, and the following lemma to the matrices $\bA \gets \bstP_r \bhatA$ and $\bB \gets \bstQ_r \bhatB$:
\end{comment}


\subsection{Balancing}
\begin{proposition}\label{prop:existence_of_balanced} Suppose that $\bA \in \R^{n \times r}$ and $\bB \in \R^{m \times r}$ are two-rank $r$ matrices with $\bM = \bA\bB^\top$. Then if
\begin{align*}
\|\bSigma_A \bSigma_B\|_{\fro} - \| \bSigma_M\|_{\fro} + 2\|\bSigma_A\|\|\bSigma_A - \bSigma_B\|_{\fro} \le \min\left\{\frac{\sigma_r(\bM)}{21},\frac{\sigma_r(\bM)^2}{21^2\|\bSigma_A^2\|_{\fro} }\right\}
\end{align*}
then there exist a  balanced $(\btilA,\btilB)$ and an $\bR$ such that $(\bA \bR, \bB \bR^{-\top}) = (\btilA,\btilB)$, such that
\begin{align*}
\frac{1}{2} \le \sigma_{r}(\bR) \le \|\bR\| \le 2.
\end{align*}
\end{proposition}


\begin{lemma}\label{lemma:inner_fact} Let $\bA, \bA' \in \R^{n \times r}$ and $\bB,\bB' \in \R^{m \times r}$ all have rank $r$ and satisfy $\bA \bB^\top = (\bA')(\bB')^\top $. Then for any $\bR_A \in \R^{r \times r}$ for which $\bA \bR_A = \bA'$ and $\bB \bR_B = \bB'$, for $ \bR_B = \bR_A^{-\top} $.
\end{lemma}



\begin{comment}\begin{lemma} Let $\bSigma$ be a real symmetric matrix. Then $\bSigma$ admits  a spectral decomposition $\bU \bD \bU^\top$, where $\det(\bU) = 1$. 
\end{lemma}
\begin{proof} Let $\bU \bD \bU^\top$ be a spectral decomposition of $\bSigma$. Since $\bU$ is real orthogonal, either $\det(\bU) = 1$, or else $\det(\bU) = -1$. If the former, we are done. If the latter, let $\bD_{1,-}$ be the diagonal matrix with $-1$ on the first diagonal, and $1$ else where. Clearly $\bD = \bD_{1,-} \bD \bD_{1,-} = \bD_{1,-} \bD \bD_{1,-}^\top$. Hence, $(\bU \bD_{1,-})\bD(\bU \bD_{1,-})^\top$ gives a spectral decomposition, and $\det(\bU \bD_{1,-}) = \det(\bD_{1,-})\det(\bU) = -\det(\bU) = 1$.
\end{proof}
\begin{lemma} Let $\bU \in \bO(r)$ have $\det(\bU) = 1$. Then, there exists some $\bU^{1/2} \in \bO(r)$
\end{lemma}
\end{comment}

\newcommand{\bcircM}{\bM_{\circ}}
\newcommand{\bcircQ}{\bQ_{\circ}}
\newcommand{\bsqM}{\bM_{\square}}

\begin{lemma}\label{lem:balance} Suppose that $\bA \in \R^{n \times r}$ and $\bB \in \R^{m \times r}$ are two-rank $r$ matrices with $\bM = \bA\bB^\top$. Further, suppose 
\begin{align*}
\| \bSigma_M - \bSigma_A \bSigma_B \|_{\fro} + 2\|\bA\|\|\bSigma_A - \bSigma_B\|_{\fro} + \| \bSigma_A^2 \bO_M - \bSigma_A \bO_M \bSigma_A\|_{\fro} \le \frac{\sigma_r(\bM)}{7 },
\end{align*}
where $\bO_M := \bV_A^\top \bV_B$. Then, there exist a  balanced $(\btilA,\btilB)$ and an $\bR$ such that $(\bA \bR, \bB \bR^{-\top}) = (\btilA,\btilB)$, such that
\begin{align*}
\frac{1}{2} \le \sigma_{r}(\bR) \le \|\bR\| \le 2.
\end{align*}
\end{lemma}

\begin{lemma}\label{lem:thing} Let $\bO \in \bbO(r)$, and let $\bSigma$ be a diagonal matrix. Then
\begin{align*}
2c_{\min}\left(\|\bSigma^2\|_{\fro}^2 - \| \bSigma \bO \bSigma\|^2_{\fro} \right)\le \|\bSigma \bO\bSigma - \bSigma^2 \bO\|_{\fro}^2 &\le 2\left(\|\bSigma^2\|_{\fro}^2 - \| \bSigma \bO \bSigma\|^2_{\fro} \right),
\end{align*}
where $c_{\min} = \frac{\lambda_{\min}(\bSigma)^2}{(\lambda_{\min}(\bSigma)+\lambda_{\max}(\bSigma))^2}. $
\end{lemma}


\begin{proof}[Proof of \Cref{prop:existence_of_balanced}]
From \Cref{lem:thing}, the conclusion of \Cref{lem:balance} holds as soon as
\begin{align}
\| \bSigma_M - \bSigma_A \bSigma_B \|_{\fro} + 2\|\bA\|\|\bSigma_A - \bSigma_B\|_{\fro} + \sqrt{2\left(\|\bSigma_A^2\|_{\fro} - \| \bSigma_A \bO_M \bSigma_A\|^2_{\fro} \right)} \le \frac{\sigma_r(\bM)}{7 }. \label{eq:thing_balance_intermediate}
\end{align}
\begin{align*}
\left(\|\bSigma_A^2\|_{\fro}^2 - \| \bSigma_A \bO \bSigma_A\|^2_{\fro} \right) &=\left(\|\bSigma_A^2\|_{\fro} - \| \bSigma_A \bO \bSigma_A\|_{\fro} \right)\left(\|\bSigma_A^2\|_{\fro} +\| \bSigma_A \bO \bSigma_A\|_{\fro} \right) \\
&\overset{(i)}{\le} 2\|\bSigma_A^2\|_{\fro} \left(\|\bSigma_A^2\|_{\fro} - \| \bSigma_A \bO \bSigma_A\|_{\fro} \right) \tag{\Cref{lem:von_neuman_one}}\\
&= 2\|\bSigma_A^2\|_{\fro} \left(\|\bSigma_A^2\|_{\fro} - \| \bSigma_A \bO \bSigma_B\|_{\fro} + \|\bSigma_A \bO(\bSigma_A - \bSigma_B)\|_{\fro}\right)\\
&= 2\|\bSigma_A^2\|_{\fro} \left(\|\bSigma_A^2\|_{\fro} - \| \bSigma_M\|_{\fro} + \|\bSigma_A \bO(\bSigma_A - \bSigma_B)\|_{\fro}\right)\\
&\le 2\|\bSigma_A^2\|_{\fro} \left(\|\bSigma_A^2\|_{\fro} - \| 
\bSigma_M\|_{\fro} + \|\bSigma_A\|\|\bSigma_A - \bSigma_B\|_{\fro} \right)\\
&\le 2\|\bSigma_A^2\|_{\fro} \left(\|\bSigma_A \bSigma_B\|_{\fro} - \| \bSigma_M\|_{\fro} + 2\|\bSigma_A\|\|\bSigma_A - \bSigma_B\|_{\fro} \right),
\end{align*}
where in $(i)$ we apply \Cref{lem:von_neuman_sq} with $\bA \gets \bA$ and $\bB \gets \bA \bO^\top$.  Defining the term
\begin{align*}
E := \|\bSigma_A \bSigma_B\|_{\fro} - \| \bSigma_M\|_{\fro} + 2\|\bSigma_A\|\|\bSigma_A - \bSigma_B\|_{\fro},
\end{align*}
and subsituting the above into \Cref{eq:thing_balance_intermediate}, is is enough that
\begin{align*}
E + 2\sqrt{E \|\bSigma_A^2\|_{\fro}}\le \frac{1}{7 \sigma_r(\bM)}.
\end{align*}
Nonnegativity of $E$ is a consequence of \Cref{lem:von_neuman_one}. A sufficient condition is that $E \le \frac{\sigma_r(\bM)}{21}$, and $2\sqrt{E \|\bSigma_A^2\|_{\fro}} \le \frac{2\sigma_r(\bM)^2}{21}$, for which it is enough that $E \le \frac{\sigma_r(\bM)^2}{21^2 \|\bSigma_A^2\|_{\fro}}$. The lemma follows. 
\end{proof}

\subsubsection{Saturation}
\begin{definition} We say $(\bA,\bB) \in \R^{n \times r_0}\times \R^{m \times r_0}$ are \emph{$(r,\epsilon,\nu)$-saturated} given $r \in \N$, $\epsilon > 0$ and $\nu \in \R_{> 0}^r$ if
\begin{itemize}
    \item[(a)] $\|\bA\bB^\top\|_{\fro} \ge \|\nu\| - \epsilon$.
    \item[(b)] For all $i \in [r]$ $\max\{\sigma_i(\bA)^2,\sigma_i(\bB)^2\} \le \nu_i$
    \item[(c)] $\rank(\bA), \rank(\bB) \le r$. 
\end{itemize}
We say they are $(\epsilon,\nu)$-fully saturated in the special case that $r_0 = r$. 
\end{definition}



\begin{lemma}\label{lem:saturated_balance} Let $(\bA,\bB)$ be $(\nu,\epsilon)$-fully-saturated, and let $\bSigma_A,\bSigma_B$ denote the matrices consisting of their respect top $r$-singular values. Then
\begin{itemize}
	\item[(a)] $\fronorm{\bSigma_A^2} \le \|\nu\|$.
	\item[(b)] $\|\bM\|_{\fro} \le \|\bSigma_A\bSigma_B\|_{\fro} \le \|\bM\|_{\fro}  + \epsilon$. 
    \item[(c)] If $\epsilon < 2\nu_r^2/\|\nu\|$, then $\rank(\bA) = \rank(\bB) = r$. 
    \item[(c)] $\|\bSigma_A\|\|\bSigma_A - \bSigma_B\|_{\fro} \le 2\epsilon\frac{\nu_1^{1/2}\|\nu\|}{\nu_r^{3/2}}$ 
    %$\|\bSigma_A^2 - \bSigma_B^2\|_{\fro} \le 2\epsilon\frac{\|\nu\|}{\nu_r^{3/2}}$\\
     
\end{itemize}

\end{lemma}

\begin{proof} By \Cref{prop:existence_of_balanced}, it suffices to show that
\begin{align*}
\|\bSigma_A \bSigma_B\|_{\fro} - \| \bSigma_M\|_{\fro} + 2\|\bSigma_A\|\|\bSigma_A - \bSigma_B\|_{\fro} \le \min\left\{\frac{\sigma_r(\bM)}{21},\frac{\sigma_r(\bM)^2}{21^2\|\bSigma_A^2\|_{\fro} }\right\}
\end{align*}
By \Cref{lem:saturated_balance}, it is enough that
\begin{align*}
\epsilon + 2\epsilon\frac{\nu_1^{1/2}\|\nu\|}{\nu_r^{3/2}} \le \min\left\{\frac{\sigma_r(\bM)}{21},\frac{\sigma_r(\bM)^2}{21^2\|\nu\| }\right\}
\end{align*}
Since $\|\nu\| \ge \nu_r$,  and $\sigma_r(\bM) \le \sigma_1(\bM)\le \sigma_1(\bA)\sigma_1(\bB) \le \|\nu\|$, it is it suffics that
\begin{align*}
\epsilon \le \frac{\nu_r^{3/2}\sigma_r(\bM)^2}{3\cdot 21^2\|\nu\|^2 \nu_1^{1/2} }. 
\end{align*}
\end{proof}

\begin{proof}[Proof of\Cref{lem:saturated_balance}] We prove each part in order.
\paragraph{Part (a).} We have $\fronorm{\bSigma_A^2}^2 = \sum_{i} \sigma_i(\bA)^4 \le \sum_i \nu_i^2 = \|\nu\|^2$.

\paragraph{Part (b).} That $\bM = \bA\bB^\top$ satisfies $\|\bM\|_{\fro} \le \|\bSigma_A \bSigma_B\|_{\fro}$ is a direct consequence of \Cref{lem:von_neuman_sq}. To prove the more second bound, we observe that since 
\begin{align*}
\|\bSigma_A \bSigma_B\|_{\fro}^2 = \sum_{i}\sigma_i(\bA)^2\sigma_i(\bB)^2 \le \sum_{i}\nu_i^2 = \|\nu\|^2.
\end{align*}
Hence, by the definition of saturation:
\begin{align*}
\|\bSigma_A \bSigma_B\|_{\fro}  \le \|\nu\| \le \|\bM\| + \epsilon. 
\end{align*}

\paragraph{Set up for parts (c) and (d). }  Define $\barnu_{i} := \max\{\sigma_i(\bA)^2,\sigma_i(\bB)^2\}$ 
and $\ubarnu_{i} = \min\{\sigma_i(\bA)^2,\sigma_i(\bB)^2\}$. From Von-Neuman's trace inequality \Cref{lem:von_neuman_sq}, we have
\begin{align*}
\|\bA\bB\|_{\fro}^2 &\le \sum_{i=1}^n \sigma_i(\bA)^2\sigma_i(\bB)^2 = \sum_{i=1}^n \barnu_{i}\ubarnu_{i} \le \sum_{i=1}^r \nu_{i}\ubarnu_{i}\\
&= \|\nu\|^2 - \sum_{i=1}^r \nu_{i}(\nu_i-\ubarnu_{i})
\end{align*}
Since $\|\bA\bB\|_{\fro}^2 \ge (\|\nu\|-\epsilon)^2 \ge (1 - 2\epsilon\|\nu\|$,  so that 
\begin{align}
\sum_{i=1}^r \nu_{i}(\nu_i-\ubarnu_{i}) \le 2\epsilon\|\nu\| \label{eq:something}
\end{align}

\paragraph{Part (c)}. Note in particular that if $\min\{\rank(\bA),\rank(\bB)\} < r$, we must have $\ubarnu_i = 0$ for some $i$, which $\nu_r^2 \le \nu_i^2 \le 2\epsilon \|\nu\|$, so $\min\{\rank(\bA),\rank(\bB)\} =r$ whenever $\epsilon < \nu_r^2/\|\nu\|/2$. This proves part (a).

\paragraph{Part (d)} We can bound
\begin{align*}
\|\bSigma_A - \bSigma_B\|_{\fro}^2 &= \sum_{i=1}^r (\sigma_i(\bA) - \sigma_i(\bB))^2 = \sum_{i=1}^r (\max\{\sigma_i(\bA),\sigma_i(\bB)\} - \min\{\sigma_i(\bA)^2,\sigma_i(\bB)^2\})^2 
\\
&= \sum_{i=1}^r (\sqrt{\barnu_i} - \sqrt{\ubarnu_i})^2 \le \sum_{i=1}^r (\sqrt{\nu_i} - \sqrt{\ubarnu_i})^2\\
&= \sum_{i=1}^r \frac{(\nu_i - \ubarnu_i)^2}{(\sqrt{\nu_i}+\sqrt{\ubarnu_i})^2} \le \nu_r^{-1}\sum_{i=1}^r (\nu_i - \ubarnu_i)^2\\
& \le \nu_r^{-1}(\sum_{i=1}^r \nu_i - \ubarnu_i)^2  \le \nu_r^{-3}(\sum_{i=1}^r \nu_i(\nu_i - \ubarnu_i))^2.
\end{align*}
Hence, combining with \Cref{eq:something},
\begin{align*}
\|\bSigma_A - \bSigma_B\|_{\fro}^2 \le \sum_{i=1}^r \nu_{i}(\nu-\ubarnu_{i}) \le 4\epsilon^2\frac{\|\nu\|^2}{\nu_r^3},
\end{align*}
as needed.

\end{proof}

\subsection{New Shit}
Let $\bA,\bB$ be two matrices, with $\bA \in \R^{n \times r}, \bB \in \R^{m \times r}$, $\rank(\bA) = \rank(\bB) = r$. 



\begin{lemma}[Rank] Suppose
\end{lemma}
\begin{proof} From \Cref{lem:von_neuman_sq}
\end{proof}


\begin{lemma}\label{lem:reduction_to_rank_r} Let$(\bA,\bB) \in \R^{n \times r_0}\times \R^{m \times r_0}$ be $(r,\epsilon,\nu)$-saturated. Then
\begin{align*}
\fronorm{\bA\bB^\top - \bcircM}^2 &\le  16\epsilon^2\frac{\|\nu\|^2}{\nu_r^2},
\end{align*}
where the matrix $\bcircM$ is constructed as follows: (a) write out $\bA = \bU_A \bSigma_A \bV_A^\top$ and $\bB = \bU_B \bSigma_B \bV_B^\top$ as a compact SVD, (b) let $\bU_Q \bSigma_Q \bV_Q^\top$ denote the SVD of  $\bQ := \bV_A^\top \bV_B$, and (c) set 
\begin{align*}\bcircM := \bU_A \bSigma_A (\bU_Q\bV_Q^\top) \bSigma_B \bU_B^\top
\end{align*}
\end{lemma}


\subsection{Proofs}
\begin{proof}[Proof of \Cref{lem:von_neuman_sq}]
\begin{align*}
\sum_{i=1}^r \sigma_i(\bM)^2 &= \trace( \bM\bM^\top) = \trace(\bA \bB^\top \bB \bA^\top) {}= \trace(\bA\bA^\top \cdot \bB\bB^\top)\\
&\le \|\bA\bA^\top \cdot \bB\bB^\top\|_{\mathrm{nuc}}\\
&= \sum_{i=1}^r \sigma_i(\bA\bA^\top \cdot \bB\bB^\top)\\
&\le \sum_{i=1}^r \sigma_i(\bA\bA^\top)  \sigma_i(\bB\bB^\top) \tag{\Cref{lem:von_neuman_one}}\\
&= \sum_{i=1}^r \sigma_i(\bA)^2  \sigma_i(\bB)^2. 
\end{align*}
To obtain the consequence, we observe that $\sum_{i=1}^r \sigma_i(\bM)^2 = \|\bM\|_{\fro}^2$, and  $\sum_{i=1}^r \sigma_i(\bA)^2  \sigma_i(\bB)^2 = \|\bSigma_A \bSigma_B\|_{\fro}^2$. 
\end{proof}
\begin{proof}[Proof of \Cref{lemma:inner_fact}] 
    Since $\bA \bB^\top = (\bA')(\bB')^\top$ and all terms are rank $r$ and have inner dimnsion $r$, there exists an $\bR_B$ for which $\bB' = \bB\bR_B$. We show that$\bR_A  \bR_B^\top = \eye_r$.

    We must have that $\bA \bR_A \bR_B^\top (\bB)^\top = \bA' (\bB')^\top = \bA\bB^\top$. Hence, for any vectors $\bv \in \R^n, \bw \in \R^m$, we have
    \begin{align*}
    \trace(\bA^\top \bv \bw^\top \bB) =  \bv^\top \bA \bR_A  \bR_B^\top\bB^\top \bw  = \trace(\bB^\top \bw \bv^\top \bA  \cdot \bR_A  \bR_B^\top )
    \end{align*}
    The above can be reformulated as
    \begin{align*}
    \trace(\bX (\eye_r - \bR_A  \bR_B^\top)  ) = 0, \quad \forall \bX \in \mathrm{span}\{\bB^\top \bw \bv^\top \bA  : \bv \in \R^n,\bw^\top \in \R^m \}.
    \end{align*}
    Since $\bA,\bB$ are rank $r$, the above $\bX$'s span all of $\R^{r \times r}$, implying $\bR_A  \bR_B^\top = \eye_r$.
\end{proof}

\begin{proof}[Proof of \Cref{lem:reduction_to_rank_r}] 
    Write out $\bA = \bU_A \bSigma_A \bV_A^\top$ and $\bB = \bU_B \bSigma_B \bV_B^\top$ as a compact SVD, with $\bSigma_A \in \R^{r \times r}$. Define the matrix $\bQ := \bV_A^\top \bV_B \in \R^{r \times r}$, and let $\bQ = \bU_Q \bSigma_Q \bV_Q^\top$ denote the compact SVD of $\bQ \in \R^{r \times}$. We consider $\bcircQ:= \bU_Q\bV_Q^\top$. Set $\bcircM := \bU_A \bSigma_A\bcircQ\bSigma_{B}\bU_B^\top$. Then
    \begin{align*}
    \fronorm{\bA\bB^\top - \bcircM}^2 &= \fronorm{\bU_A \bSigma_A \bV_A^\top \bV_B \bSigma_B \bU^\top - \bU_A \bSigma_A\bcircQ\bSigma_{B}\bU_B^\top}^2\\
    &= \fronorm{\bU_A \bSigma_A (\underbrace{\bV_A^\top \bV_B}_{=\bQ} - \bcircQ) \bSigma_B \bU^\top_B}^2\\
    &= \fronorm{\bU_A \bSigma_A (\bU_Q \bSigma_Q \bV_Q^\top - \bU_Q\bV_Q^\top) \bSigma_B \bU_B^\top}^2\\
    &= \fronorm{\bU_A \bSigma_A \bU_Q (\bSigma_Q  - \eye_r) \bV_Q^\top  \bSigma_B \bU_B^\top}^2\\
    &= \fronorm{ \bSigma_A \bU_Q (\bSigma_Q  - \eye_r) \bV_Q^\top  \bSigma_B}\\
    &= \langle \bSigma_A \bU_Q (\bSigma_Q  - \eye_r) \bV_Q^\top  \bSigma_B, \bSigma_A \bU_Q (\bSigma_Q  - \eye_r) \bV_Q^\top  \bSigma_B\rangle\\
    &= \langle \bSigma_A^2 \bU_Q (\bSigma_Q  - \eye_r) \bV_Q^\top  ,  \bU_Q (\bSigma_Q  - \eye_r) \bV_Q^\top  \bSigma_B^2\rangle\\
    &\le \|\bSigma_A^2 \bU_Q (\bSigma_Q  - \eye_r) \bV_Q^\top\|_{\fro} \cdot \|\bU_Q (\bSigma_Q  - \eye_r) \bV_Q^\top  \bSigma_B^2\|_{\fro}\\
    &= \|\bSigma_A^2 \bU_Q (\bSigma_Q  - \eye_r) \|_{\fro} \cdot \| (\bSigma_Q  - \eye_r) \bV_Q^\top  \bSigma_B^2\|_{\fro}. 
    \end{align*}
    Next, letting $\nu_{i,A} = \lambda_i(\bSigma_A)^2$, $\delta_i = 1-\lambda_i(\bSigma_Q)$, and $\bL_{ij,U} = (\bU_Q)_{ij}^2$, we have
    \begin{align*}
    \|\bSigma_A^2 \bU_Q (\bSigma_Q  - \eye_r) \|_{\fro}^2 = \sum_{i,j} \nu_{i,A}^2 \delta_j^2 \bL_{ij,U}.
    \end{align*}
    Similarly, with $\nu_{i,B} = \lambda_i(\bSigma_B)^2$,  and $\bL_{ij,V} = (\bV_Q)_{ji}^2$ (notice the reversal of indices), 
    \begin{align*}
    \|(\bSigma_Q  - \eye_r) \bV_Q^\top  \bSigma_B^2 \|_{\fro}^2 = \sum_{i,j} \nu_{i,B}^2 \delta_j^2 \bL_{ij,V}. 
    \end{align*}
    Hence, for any $\nu_i \ge \max\{\nu_{i,A},\nu_{i,B}\}$ and $\bL_{i,j,U} = \frac{1}{2}(\bL_{ij,U} + \bL_{ij,V})$, we have
    \begin{align*}
    \fronorm{\bA\bB^\top - \bcircM}^4 &\le (\sum_{i,j} \nu_{i,A}^2 \delta_j^2 \bL_{ij,U})(\sum_{i,j} \nu_{i,B}^2 \delta_j^2 \bL_{ij,V}) \le (\sum_{i,j} \nu_{i}^2 \delta_j^2 \bL_{ij,U})(\sum_{i,j} \nu_{i}^2 \delta_j^2 \bL_{ij,V})\\
    &\le (\sum_{i,j} \nu_{i}^2 \delta_j^2 \bL_{ij})^2 \tag{AM-GM}
    \end{align*}
    and hence
    \begin{align}
    \fronorm{\bA\bB^\top - \bcircM}^2 &\le E_0 := \sum_{i,j} \nu_{i}^2 \delta_j^2 \bL_{ij}  \label{eq:fro_diff_bound}
    \end{align}

    By a similar calculation, and considering any $\nu$ $\nu_i \ge \max\{\nu_{i,A},\nu_{i,B}\}$ $\bL_{i,j,U} = \bL_{ij,U} + \bL_{ij,V}$, we have we have
    \begin{align*}
    \|\bA\bB^\top\|_{\fro}^4 &\le  (\sum_{i,j} \nu_{i,A}^2 (1-\delta_j)^2 \bL_{ij,U}) \cdot (\sum_{i,j} \nu_{i,B}^2 (1-\delta_j)^2 \bL_{ij,V})\\
    &\le  (\sum_{i,j} \nu_{i}^2 (1-\delta_j)^2 \bL_{ij,U}) \cdot (\sum_{i,j} \nu_{i}^2 (1-\delta_j)^2 \bL_{ij,V})\\
    &\le  (\sum_{i,j} \nu_{i}^2 (1-\delta_i) \bL_{ij,U}) \cdot (\sum_{i,j} \nu_{i}^2 (1-\delta_k) \bL_{ij,V})\\
    &=  \|\nu\|^4 - \|\nu\|^2\left(\sum_{i,j} \underbrace{(\bL_{ij,U} + \bL_{ij,V})}_{=2\bL_{ij}} \nu_{i}^2 \delta_j\right)  +  (\sum_{i,j} \nu_{i}^2 \delta_i \bL_{ij,U})(\sum_{i,j} \nu_{i}^2 \delta_i \bL_{ij,V}) \\
    &=  \|\nu\|^4 - 2\|\nu\|^2\underbrace{\left(\sum_{i,j} \bL_{ij} \nu_{i}^2 \delta_j\right)}_{:= E_1}  +  \underbrace{\left(\sum_{i,j} \nu_{i}^2 \delta_j \bL_{ij}\right)^2}_{ = E_1^2} \tag{AM-GM}\\
    &=  \|\nu\|^4 - 2\|\nu\|^2 E_1  +  E_1^2\\
    &\le \|\nu\|^4 - \|\nu\|^2 E_1,
    %&=  (\sum_{i,j} \nu_{i,A}^2  \bL_{ij,U}) \cdot (\sum_{i,j} \nu_{i,B}^2  \bL_{ij,V}) + (\sum_{i,j} \nu_{i,A}^2  \delta_i^2 \bL_{ij,U}) \cdot (\sum_{i,j} \nu_{i,B}^2  \delta_j^2 \bL_{ij,V})
    \end{align*}
    where the last line uses
    $0 \le E_1 = \sum_{i,j} \bL_{ij} \nu_{i}^2 \delta_j \le \sum_{i,j} \bL_{ij} \nu_{i}^2 \le \|\nu\|^2$, so that $E_1^2  - 2\|\nu\|^2 E_1  = E_1(E_1 - 2\|\nu\|^2)\le -\|\nu\|^2 E_1$.By the assumption of the theorem, we have 
    \begin{align*}
    \|\bA\bB^\top\|_{\fro} \ge (\|\nu\| - \epsilon)^4. 
    \end{align*}
    Then, we must have $\|\nu\|^4 - \|\nu\|^2 E_1  \ge (\|\nu\| - \epsilon)^4 \ge \|\nu\|^4 - 4\|\nu\|^3 \epsilon$, so that
    \begin{align}
     E_1 \le 4\epsilon\|\nu\| \label{eq:Eone_bound}
    \end{align}

    To conclude, we compare terms $E_1$ and $E_0$. To this end, set $\alpha_j := \sum_{ij} \nu_i^2 \bL_{ij}$. We above that, since $\sum_{i=1}^r\bL_{ij} = 1$, and since we order $\nu_i$ is descending order without loss of generality, we ahve $\nu_r^2 \le \alpha_j \le \nu_1^2$. We now express
    \begin{align*}
     E_0 &:= \sum_{i,j} \nu_{i}^2 \delta_j^2 \bL_{ij}  = \sum_j \alpha_j \delta_j^2, \quad E_1 := \sum_{i,j} \nu_{i}^2 \delta_j \bL_{ij}  = \sum_j \alpha_j \delta_j.
    \end{align*}
    Thus, 
    \begin{align*}
    E_0  &= \sum_{j}(\sqrt{\alpha} \delta_j)^2 \le (\sum_{j}\sqrt{\alpha_j} \delta_j)^2 = \sum_{j}(\sqrt{\alpha} \delta_j)^2 \le (\frac{1}{\alpha_r^{1/2}}\sum_{j}\alpha_j \delta_j)^2 = \frac{E_1^2}{\alpha_r} = \frac{E_1^2}{\nu_r^2},
    \end{align*}

    Therefore, from \Cref{eq:fro_diff_bound}, we have
    \begin{align*}
    \fronorm{\bA\bB^\top - \bcircM}^2 &\le \frac{E_1^2}{\nu_r^2} \le \frac{16\epsilon^2\|\nu\|^2}{\nu_r^2}
    \end{align*}
\end{proof}
\begin{proof}[Proof of \Cref{lem:balance}] 
    Let's write our the compact SVDs of $\bA,\btilA$ as 
    \begin{align*}
    \bA = \bU_A \bSigma_A \bV_A \quad \btilA = \btilU_M \bSigma_M^{1/2}, \
    \end{align*}
     Observe that since $\bU_A$ and $\btilU_A$ are orthonormal matrices which span the space space, there exist some orthonormal matrix $\bN_A$ such that $\bU_A = \bU_M \bN_A$. Specifically, we can solve
    \begin{align*}
    \eye_r = \bU_A^\top \bU_A = (\bU_A^\top \bU_M)\bN_A, \quad \bN_A = \bu_M^\top \bU_A.
    \end{align*}
    \begin{align*}
    \bA = \btilU_A \bO_A \bSigma_A \bV_A = \btilU_A \bSigma_M^{1/2}  \underbrace{\bSigma_M^{-1/2}\bN_A \bSigma_A \bV_A}_{=\bR^{-1}} = \btilA \bR^{-1}.
    \end{align*}
    Note that by \Cref{lemma:inner_fact}, the fact that $\bA \bR = \btilA$ ensures that also $\bB \bR^{-\top}= \btilB$. For any other orthonormal matrix $\bO \in \bbO(r)$, 
    \begin{align*}
    \bR &= \bSigma_M^{-1/2}\bN_A \bSigma_A \bV_A\\
    &= \bSigma_M^{-1/2} \bU_M^\top \bU_A \bSigma_A \bV_A\\
    &= \bSigma_M^{-1/2} \bU_M^\top (\bU_M \bSigma_M^\top \bO -  \bU_A \bSigma_A^{1/2}) \bV_A
    \end{align*}
    and thus, setting $\epsilon_{R} := \sigma_{r}(\bM)^{-1/2}\cdot \inf_{\bO} \|\bU_M \bSigma_M^\top \bO -  \bU_A \bSigma_A^{1/2})\|_{\op}$, 
    \begin{align*}
    &1 - \epsilon_R \le \sigma_{\min}(\bR^{-1}) \le \sigma_{\max}(\bR_A^{-1}) \le 1 + \epsilon_R. 
    \end{align*}
    To bound $\epsilon_R$, set $\bX = \bU_A \bSigma_M^{1/2}$ and $\bY^\top = \bSigma_M^{1/2} \cdot \bV_A \bV_B^\top \bU_B^\top$, $\bM_{\square} = \bX\bY^\top$. Thus, there exist some term $\Delta$ such that 
    \begin{align*}
    \|\bU_A \bSigma_M^{1/2} - \bU_M \bSigma_M^{1/2} \bO\|_{\op} \le \|\bU_A \bSigma_M^{1/2} - \bU_M \bSigma_M^{1/2} \bO\|_{\fro}\le \sqrt{2}\cproc\frac{ \|\bM_{\square,2}- \bM\|_{\fro}}{\sigma_r(\bM)^{1/2}},
    \end{align*}
    provided $\|\bM_{\square}- \bM\|_{\fro} \le \sigma_r(\bM)/2$. Hence, we can bound
    \begin{align*}
    \epsilon_A \le \sqrt{2}\cproc\frac{ \|\bM_{\square}- \bM\|_{\fro}}{\sigma_r(\bM)} \le \frac{7}{2}\frac{ \|\bM_{\square}- \bM\|_{\fro}}{\sigma_r(\bM)}
    \end{align*}
    Hence, if $\frac{ \|\bM_{\square}- \bM\|_{\fro}}{\sigma_r(\bM)} \le 1/7$, we can take $\epsilon_R = 1/2$, and thus 
    \begin{align*}
    1/2 \le \sigma_{\min}(\bR_A^{-1}) \le \sigma_{\max}(\bR_A^{-1}) \le 2, \quad  \text{so that } 1/2 \le \sigma_{\min}(\bR_A) \le \sigma_{\max}(\bR_A) \le 2
    \end{align*}
    Lastly, let us decompose 
    \begin{align*}
    \|\bM_{\square}- \bM\|_{\fro} &= \|\bU_A \bSigma_M \cdot \bV_A \bV_B^\top \bU_B^\top - \bM\|_{\fro}\\
    &\le \|\bU_A (\bSigma_M - \bSigma_A \bSigma_B) \cdot \bV_A \bV_B^\top \bU_B^\top\|_{\fro} \\
    &\qquad+  \|\bU_A \bSigma_A \bSigma_B\cdot \bV_A \bV_B^\top \bU_B^\top -  \bU_A \bSigma_A \bV_A \bV_B^\top \bSigma_B\cdot  \bU_B^\top \\
    &\quad+ \underbrace{\|\bU_A \bSigma_A \bV_A \bV_B^\top \bSigma_B\cdot  \bU_B^\top - \bM\|_{\fro}}_{=\|\bA \bB^\top- \bM\|_{\fro} = 0}\\
    &= \| \bSigma_M - \bSigma_A \bSigma_B \|_{\fro} + \| \bSigma_A \bSigma_B\cdot \bV_A \bV_B^\top - \bSigma_A \bV_A \bV_B^\top \bSigma_B\|_{\fro} \\
    &\le \| \bSigma_M - \bSigma_A \bSigma_B \|_{\fro} + 2\|\bSigma_A\|_{\op}\|\bSigma_A - \bSigma_B\|_{\fro} + \| \bSigma_A^2 \bO_A - \bSigma_A \bO_M \bSigma_A\|_{\fro}, 
    \end{align*}
    where $\bO_M = \bV_A \bV_B^\top$. 
\end{proof}


\begin{proof}[Proof of \Cref{lem:thing}] 

        By conjugating by a diagonal-sign matrix, we may assume without loss of generality that $\bSigma \succeq 0$.
    \begin{align*}
    \veps =  \|\bSigma^2\|_{\fro} - \|\bSigma \bO \bSigma\|_{\fro}^2,
    \end{align*}
    Further, set $\nu_i = \bSigma_i^2$ as $\nu_{i}$ and $\bL_{ij} = \bO_{ij}^2$, so that
    \begin{align*}
    \|\bSigma \bO\bSigma\|_{\fro}^2 = \sum_{i,j=1}^r \bO_{ij}^2 \nu_i \nu_j
    \end{align*}
    Let $\bL_{ij} = \bO_{ij}^2$. Then, $\bL$ is a doubly stochastic $r \times r$ matrix, and 
    \begin{align}
    \sum_{i=1}^r \nu_i^2 - \sum_{i,j=1}^r \bL_{ij} \nu_i \nu_j = \veps \label{eq:veps_cond_L}
    \end{align}

    \begin{claim}\label{claim:L_sym_doubstoch} Suppose $\bL$ is doubly stochastic and symmetric and satisfies \Cref{eq:veps_cond_L}. Then, 
    \begin{align*} 
    \sum_{i < j} (\nu_i-\nu_j)^2\bL_{ij} = \veps.
    \end{align*}
    \end{claim}
    \begin{proof} Let $\scrLsym$ denote the subset of $\scrL'$ which is symmetric. Define the operator for $\bL' \in \scrLsym$ given by $\Psi_{ij}(\bL') = \bL' + \bL_{ij}(e_ie_i^\top + e_je_j^\top - e_ie_j^\top -e_je_i^\top)$. One can check that for $i = j$, $\Psi_{ij}$ is just the identity, whereas for all $i \ne j$, $\Psi_{ij}$ maps $\scrLsym \to \scrLsym$ (preservation of symmetry is clear, summation of rows to one is clear, symmetry of $\bL'$  ensures nnonegativity of the entries of $\Psi_{ij}(\bL')$). Consider pairs of $(i,j), 1 \le i \le j \le r$ in lexicographic order, and  for $(i,j) \ne (1,1)$, let $(i,j) - 1$ denote the predecessor of $(i,j)$ in this order. Define a sequence $\bL_{(i,j)}$ via
    \begin{align*}
    \bL_{(i,j)} = \Psi_{ij}(\bL_{(i,j)-1}), \quad \bL_{(1,1)} = \bL, \quad \bL_{\star} := \bL_{r-1,r}.
    \end{align*} 
    We find then verify inductively that, for all $1 \le i_0 \le j_0 \le r$,
    \begin{align*}
    \sum_{i,j}(\bL_{(i_0,j_0)} )_{i,j}\nu_i\nu_j &= \sum_{i,j} (\bL_{i,j}\nu_i \nu_j ) + \sum_{(i,j) \le (i_0,j_0), i \le j} (\nu_i^2 + \nu_j^2 - 2\nu_{ij}^2)\bL_{ij}\\
    &= \sum_{i,j} (\bL_{i,j}\nu_i \nu_j ) + \sum_{(i,j) \le (i_0,j_0), i < j} (\nu_i-\nu_j)^2\bL_{ij}
    \end{align*}
    In particular,
    \begin{align*}
    \sum_{i,j}(\bL_{(r,r)} )_{i,j}\nu_i\nu_j -\sum_{i,j} (\bL_{i,j}\nu_i \nu_j ) = \sum_{i < j} (\nu_i-\nu_j)^2\bL_{ij}
    \end{align*}
    Moreover, we can verify inductively that $(\bL_{(i_0,j_0)})_{i,j} =0$ for all $(i,j) \le (i_0,j_0)$, so that $\bL_{(r,r)} \in \scrLsym$ is a diagonal (using symmetry), doubly-stochastic matrix, and thus equal to the identity. Hence
    \begin{align*}
    \sum_{i < j} (\nu_i-\nu_j)^2\bL_{ij} = \sum_{i=1}^r\nu_i^2 -\sum_{i,j} (\bL_{i,j}\nu_i \nu_j ) = \veps. 
    \end{align*}

    \end{proof}
    \begin{claim} Suppose $\bL$ is doubly stochastic and  but possibly non symmetric and satisfies \Cref{eq:veps_cond_L}. Then, 
    \begin{align*} 
    \sum_{i \ne j} (\nu_i-\nu_j)^2\bL_{ij} = 2\veps.
    \end{align*}
    \end{claim}
    \begin{proof} If $\bL$ is doubly stochastic, so is $\bL^\top$, and thus so is $\bL' = \frac{1}{2}(\bL + \bL^\top)$. Apply \Cref{claim:L_sym_doubstoch} to $\bL'$ to find that
    \begin{align*}
    \veps = \sum_{i < j} (\nu_i-\nu_j)^2\bL'_{ij} &= \sum_{i < j} (\nu_i-\nu_j)^2(\bL_{ij}+\bL_{ji})/2\\
    &= \frac{1}{4}\sum_{i \ne j} (\nu_i-\nu_j)^2(\bL_{ij}+\bL_{ji})= \frac{1}{2}\sum_{i \ne j} (\nu_i-\nu_j)^2\bL_{ij}.
    \end{align*}
    \end{proof}
    Next, write (again, with $\bL_{ij}  = (\bO_{ij}^2$)
    \begin{align*}
    \|\bSigma \bO\bSigma - \bSigma^2 \bO\|_{\fro}^2 &= \sum_{i,j=1}^r (\sigma_i(\bSigma)\sigma_j(\bSigma) \bO_{ij} - \sigma_i(\bSigma_A)^2 \bO_{ij})^2\\
    &= \sum_{i,j=1}^r (\sqrt{\nu_i\nu_j}  - \nu_i)^2\bL_{ij}\\
    &=\sum_{i,j=1}^r \nu_i(\sqrt{\nu_i} - \sqrt{\nu_j})^2\bL_{ij} = \sum_{i,j=1}^r (\nu_i - \nu_j)^2\bL_{ij} \cdot \frac{\nu_i}{(\sqrt{\nu_j}+\sqrt{\nu_i})^2} \numberthis \label{eq:thing}\\
    &\le \sum_{i,j=1}^r (\nu_i - \nu_j)^2\bL_{ij} = 2\epsilon\\
    &= 2\left(\|\bSigma^2\|_{\fro}^2 - \| \bSigma \bO \bSigma\|^2_{\fro} \right)
    \end{align*}
    Moreover, from \Cref{eq:thing}, we have
    \begin{align*}
    \|\bSigma \bO\bSigma - \bSigma^2 \bO\|_{\fro}^2 \ge  \underbrace{\min_{i,j}(\frac{\nu_i}{(\sqrt{\nu_j}+\sqrt{\nu_i})^2})}_{c_{\min}} \cdot \sum_{i,j=1}^r (\nu_i - \nu_j)^2\bL_{ij} \sum_{i,j=1}^r (\nu_i - \nu_j)^2 = 2c_{\min}\left(\| \bSigma \bO \bSigma\|^2_{\fro} - \|\bSigma^2\bO\|_{\fro}^2\right).
    \end{align*}
    One can check that $c_{\min}$ is minimized for $\nu_i = \min_k \nu_{k} = \lambda_{\min}(\bSigma)^2$ and $\nu_j = \max_k \nu_k = \lambda_{\min}(\bSigma)^2$. The ratio is then
    \begin{align*}
    c_{\min} = \frac{\lambda_{\min}(\bSigma)^2}{(\lambda_{\min}(\bSigma)+\lambda_{\max}(\bSigma))^2}. 
    \end{align*}
\end{proof}
