# Supplementary material for: Tackling Combinatorial Distribution Shift: A Matrix Completion Perspective
Source: arXiv:2307.06457 source file (2023-07-28)
Supplement: Supplementary file 3 [file old_other.tex]

For any matrix $r \in \N$, and let $\bstP_r,\bstQ_r$ denote the projection to its left (resp. right) singular spaces (breaking ties arbitrarily). Similarly,  let  $\bhatP_r,\bhatQ_r$ denote the projections on its left (resp. right) singular spaces. We define the rank-$r$ SVD's of $\bstM$ and $\bhatM$, and their complements, via
\subsection{Eigendecya}

\begin{lemma} For any $k$, there exists a $k' \le k$ such that $\delst_{k'} \ge 1/k$ and 
\begin{align*}
\epsapx(k') \le \epsapx(k) + e\sqrt{k}\sigma_{k}.  
\end{align*}
$\delst_j = 1 - \frac{\sigma_{j+1}}{\sigma_j}$.
\end{lemma}
\begin{proof}  Let $k' := \max\{1 \le j \le k: \delst_j \le 1/k\}$ if $\delst_1 \le 1/k$, and $k' = 0$ otherwise.  $\sigma_{k'} \le e \sigma_{k}$. $\epsapx(k')^2 = \sum_{j=k'}^{\infty} \sigma_{j}^2 = \sum_{j=k+1}^{\infty} \sigma_{j}^2 + \sum_{j=k'}^k \sigma_j^2  = \epsapx(k) + \sum_{j=k'}^k \sigma_j^2 \le \epsapx(k) + k e \sigma_k^2$. Take square root + concavity. 
\end{proof}

\begin{claim} Let $\sigma_1 \ge \sigma_2 \ge \dots \ge \dots \ge \sigma_k$. Suppose that for some $k_1 \in [k-1]$, it holds that $\delta_j := 1 - \frac{\sigma_j}{\sigma_{j+1}} \le 1 - \frac{1}{k}$ for all $j \in \{k_1,k_1+1,\dots,k-1\}$. Then, 
\begin{align*}
\sigma_{k_1} \le e\sigma_k.
\end{align*}
\end{claim}
\begin{proof}
We have
\
\end{proof}

\begin{comment}
\begin{claim} Let $\sigma_1 \ge \sigma_2 \ge \dots \ge \dots \ge \sigma_k$. Suppose that for some $k_1 \in [k-1]$, it holds that $\delta_j := 1 - \frac{\sigma_j}{\sigma_{j+1}} \le 1 - \frac{1}{\beta j}$ for all $j \in \{k_1,k_1+1,\dots,k-1\}$. Then, 
\begin{align*}
\sigma_{k_1} \le 2(k/k_1)^{1/\beta}\sigma_k
\end{align*}
\end{claim}
\begin{proof}
Using $\delta_j \le j/\beta$, so that $(1 - \delta_j)^{-1} \le (1 - 1/j\beta)^{-1}$, the following holds for any $k_1 \ge 2$:
\begin{align*}
\sigma_{k_1} &= \sigma_k \cdot \prod_{j=k_1}^{k - 1} \frac{\sigma_j}{\sigma_{j+1}} = \sigma_k \cdot \prod_{j=k_1}^{k - 1} (\frac{\sigma_{j+1}}{\sigma_j})^{-1}\\
&= \sigma_k \cdot \prod_{j=k_1}^{k -1} (1 - \delta_j)^{-1}\\
&\le \sigma_k \cdot \prod_{j=k_1}^{k -1} (1 - \frac{1}{j\beta})^{-1}\\
&= \sigma_k \cdot \left(\prod_{j=k_1}^{k -1} (1 - \frac{1}{j\beta})^{-\beta}\right)^{1/\beta}\\
\end{align*}
Observe then that
\begin{align*}
 (1 - \frac{1}{j\beta})^{\beta} \ge 1-\frac{1}{j}, \beta \le 1 \le j. 
\end{align*}
Hence,
\begin{align*}
\sigma_{k_1} &\le \sigma_k \cdot \left(\prod_{j=k_1}^{k_1 -1} (1 - \frac{1}{j\beta})^{-\beta}\right)^{1/\beta} \\
&\le \left(\prod_{j=k_1}^{k -1} (1 - \frac{1}{j})^{-1} \right)^{1/\beta}\\
&\le \left(\prod_{j=k_1}^{k -1} \frac{j}{j-1} \right)^{1/\beta} = (\frac{k - 1}{k_1 - 1})^{1/\beta} \numberthis \label{eq:number_intermediate_k} \\
&\le (\frac{2k}{k_1})^{1/\beta} \le 2^{1/\beta} (k/k_1)^{1/\beta}.
\end{align*}
For $k_1 = 1$, we have that if $\delta_j \le 1 - \frac{1}{\beta j}$ for all $j \in [k-1]$, then 
\begin{align*}
\sigma_{1} &= (1 - \delta_1)^{-1}\sigma_{2} = (1-\beta)^{-1}\sigma_{2} \\
&\le (1-\beta)^{-1}(\frac{k - 1}{2 - 1})^{1/\beta}  \tag{\Cref{eq:number_intermediate_k}} \\
&= (1-\beta)^{-1}k^{1/\beta} = (1-\beta)^{-1}(k/1)^{1/\beta}). 
\end{align*}
Combining both cases, and using $\beta \le 1/2$,
\begin{align*}
\sigma_{k_1} \le \min\{2^{1/\beta},(1-\beta)^{-1}\}(k/k_1)^{1/\beta} \le 2(k/k_1)^{1/\beta}. 
\end{align*}
\end{proof}
\end{comment}
\subsection{More Wedin}
\mscomment{TODO: show $\|\bhatM - \bstM\|_{\fro}$ small implies $\|\bhatM_k - \bstM_k\|_{\fro}$ small. This can be achieved by a double-Wedin's theorem.  }

\begin{comment}
\subsubsection{Proof of \Cref{lem:discrete_apx}}
\mscomment{make sure these functions are uniformly bounded}
For simplicity, we exhibit a discretization for $\Fbarp$, the discretization for $\Gbarp$ is similar. Recall that we may assume with out loss of generality that the image of any lies $\fbar\in \Fbarp$ lies in the finite vector space $\R^p$.


%Since $\Fbarp$ is a finite finite, there exist some $x_0 \in \xspace$ and constant $C_0$ such that $\|\fbar(x_0)\| \le C_0$ for all $\fbar \in \Fbarp$. For each $\tau$, since $B_{\tau} := C_0\sqrt{\tau}$, and 
Fix an $x_0 \in \xspace$,  define 
\begin{align*}
\xspace_{\tau} := \{x \in \xspace: \max_{\fbar \in \Fbarp}\|f(x)\| \le B_{\tau} \}, \quad B_{\tau}= \sqrt{\tau},
\end{align*}
and consider the collect of sets of the form
\begin{align*}
\cW_{\ba,\tau} := \bigtimes_{i=1}^p\left[B_{\tau}\cdot\frac{\ba_i-1}{\tau},B_{\tau}\cdot \frac{\ba_i}{\tau}\right), \quad \ba \in\scrA_{\tau} :=  \{-\tau,1-\tau,\dots,0,1,\dots\tau+1\}^p.
\end{align*}

It is clear that for a given $\tau$ and two $\ba \ne \ba' \in \scrA_{\tau}$, $\cW_{\ba,\tau} \cap \cW_{\ba',\tau} =\emptyset$, and that $\bigcup_{\ba \in \scrA_{\tau}}\bW_{\ba,\tau} \supset \{\bv \in \R^p: \|\bv\| \le B_{\tau}\}$. In other words, the finitely-many sets $(\cW_{\ba,\tau})_{\ba \in \scrA_{\tau}}$ partition the radiu $B_{\tau}$ ball in $\bR^p$. Notice also that these are Borel sets.

Next, given $\vec{\ba} = (\ba^{(1)},\dots,\ba^{(p+1)}) \in \scrA_{\tau}^{p+1}$, let
\begin{align*}
\scrX_{\vec{\ba},\tau} &:= \{x \in \xspace_{\tau}: f(x) \in \cW_{\ba^{(p+1)},\tau} \text{ and } \,\forall k \in [p], \,\fstk(x) \in \cW_{\ba^{(k)},\tau}  \}
%\scrY_{\vec{\ba},\tau} &:= \{y \in \yspace: g(y) \in \cW_{\ba^{(p+1)},\tau} \text{ and }\, \forall k \in [p], \,\gstk(y) \in \cW_{\ba^{(k)},\tau}  \}
\end{align*}
One can check that $\scrX_{\vec{\ba},\tau} $ partitions $\scrX_{\tau}$. Since there are finitely many such sets, (without invoking the axiom of choice!) we can choose  a single representative element $x_{\vec{\ba}} \in \scrX_{\vec{\ba},\tau}$  in each of these sets, and the function
\begin{align*}
\phixtau(x) &= \begin{cases} x_{\vec{\ba}} & x \in \scrX_{\vec{\ba},\tau} \\ 
x_0 & x \notin \scrX_{\tau}
\end{cases}\\
\end{align*}
is well-defined. Notice that $\phixtau$ is also measurable: indeed, (considering the $x$-case) the image of $\phixtau$ is supported on finitely many elements $\{x_{\vec{\ba}}\}_{\vec\ba \in \scrA_{\tau}^{p+1}}\cup\{x_0\}$, and
\begin{align*}
(\phixtau)^{-1}(x_{\vec{\ba}}) =  \scrX_{\vec{\ba},\tau} = f^{-1}(\cW_{\ba^{(p+1)},\tau}) \cap \bigcap_{k=1}^p (\fstk)^{-1}(\cW_{\ba^{(k)},\tau}),
\end{align*}
which is a finite intersection of preimages of Borel sets under measurable functions. A similar computation shows $\phixtau^{-1}(x_0)$ is measurable. 

To compute the discretization error, we take $\fbar \in \Fbarp$ and use (letting $\Exp = \Exp_{\cdxone}$ as shorthand)
\begin{align*}
\lim_{\tau \to \infty}\Exp[\|\fbar - \fbar \circ \phixtau\|^2] &\le \underbrace{\lim_{\tau \to \infty}\sup_{x \in \scrX_{\tau}}\|\fbar - \fbar \circ \phixtau\|^2}_{:= T_1} + \underbrace{\lim_{\tau to \infty} \Exp[\I\{x\notin \scrX_{\tau}\}\|\fbar - \fbar \circ \phixtau\|^2]}_{:= T_2}
\end{align*}
To bound $T_1$, let  $x \in \xspace \scrX_{\tau}$. Since  $(\scrX_{\vec{\ba},\tau})$ partitions $\scrX$, there exist some $\vec{\ba}_x$ such that $x \in \scrX_{\vec{\ba}_x,\tau}$. Letting $\ba_0 := \vec{\ba}_x^{(p+1)}$, it follows that $f(x) \in \cW_{\ba_0,\tau}$. Similarly, $\phixtau(x) \in \scrX_{\vec{\ba}_x,\tau}$ by construction, so $f \circ \phixtau(x) \in  \cW_{\ba_0,\tau}$. Hence, 
\begin{align*}
\|\fbar(x) - \fbar\circ\phixtau(x)\|_2 &\le \sup_{\bv,\bv' \in \cW_{\ba_0,\tau}}\|\bv - \bv'\|_{2}\\
&\le \sup_{\bv,\bv' \in \cW_{\ba_0,\tau}}\|\bv - \bv'\|_{1} = \frac{B_{\tau} p}{\tau} = p/\sqrt{\tau}.
\end{align*}
This shows that the error term $T_1 = 0$. To bound $T_2$, note that for any $x\notin\scrX_{\tau}$, $\phixtau(x) = x_0$. Hence
\begin{align*}
\Exp[\I\{x\notin \scrX_{\tau}\}\|\fbar - \fbar \circ \phixtau\|^2] &= \Exp[\I\{x\notin \scrX_{\tau}\}\|\fbar - \fbar \circ \phixtau\|^2] \\
&= \Exp[\I\{x\notin \scrX_{\tau}\}\|\fbar(x) - \fbar(x_0)\|^2] \\
&\le \Exp[\I\{\|\fbar(x)\| \le \sqrt{\tau}\}\|\fbar(x) - \fbar(x_0)\|^2] \overset{\tau \to \infty}{\to} 0,
\end{align*}
where the convergence to zero holds since $\|\fbar(x) - \fbar(x_0)\|^2$ is integrable. This concludes the proof bounding the discretization error.

To conclude, we argue why we can choose the induced distributions $\cdxtau$ and $\cdytau$ to preserve the zero measure of any single sets $\scrX_0 \subset \scrX$ and $\scrY_0 \subset \scrY$. \mscomment{conclude this}
\end{comment}
